# Supplementary material for: High-dimensional consistency in score-based and hybrid structure learning
Source: arXiv:1507.02608 ancillary file (2018-02-03)
Supplement: Supplementary file 1 [file supplement.pdf]

# Supplement to "High-dimensional consistency in score-based and hybrid structure learning"

Preetam Nandy, Alain Hauser and Marloes H. Maathuis

This document contains supplementary information for the paper (main text) "High-dimensional consistency in score-based and hybrid structure learning" [Nandy et al., 2016].

# Contents

**1 Preliminary simulations** **2**

**2 Properties of a scoring criterion** **4**

**3 Pseudocode for GES** **4**

**4 Additional details for Example 1 of the main text** **5**
4.1 Search paths . . . . . . . . . . . . . . . . . . . . . . . . . . . . . . 5
4.2 Computation of large sample limits . . . . . . . . . . . . . . . . . . . 6
4.3 Large sample limit outputs of hill-climbing DAG search and its hybrid versions 7

**5 Empirical verification of Assumption (A5) of the main text** **8**

**6 Inclusion of a turning phase in (AR)GES** **9**

**7 Effect of the tuning parameter $\gamma_n$ on the performance ARGES-CIG** **9**

**8 CIG and CPDAG-skeleton estimation results corresponding to Section 8.3 of the main text** **11**

**9 Proofs** **11**
9.1 Proof of Theorem 4.1 of the main text . . . . . . . . . . . . . . . . . . 11
9.2 Proof of Corollary 4.1 of the main text . . . . . . . . . . . . . . . . . . 16
9.3 Proof of Theorem 4.2 of the main text . . . . . . . . . . . . . . . . . . 17
9.4 Proof of Theorem 4.3 of the main text . . . . . . . . . . . . . . . . . . 17
9.5 Proof of Lemma 5.1 of the main text . . . . . . . . . . . . . . . . . . . 18
9.6 Proof of Theorem 5.1 of the main text . . . . . . . . . . . . . . . . . . 19
9.7 Proof of Theorem 5.2 of the main text . . . . . . . . . . . . . . . . . . 20

9.8 Proof of Lemma 5.3 of the main text . . . . . . . . . . . . . . . . . . . . . . . . 23
9.9 Proof of Theorem 5.3 of the main text . . . . . . . . . . . . . . . . . . . . . . . 23
9.10 Proof of Theorem 5.4 of the main text . . . . . . . . . . . . . . . . . . . . . . 32
9.11 Proof of Theorem 6.1 of the main text . . . . . . . . . . . . . . . . . . . . . . 33
9.12 Proof of Lemma 7.1 of the main text . . . . . . . . . . . . . . . . . . . . . . . 34
9.13 Proof of Lemma 7.2 of the main text . . . . . . . . . . . . . . . . . . . . . . . 34
9.14 Proof of Theorem 7.1 of the main text . . . . . . . . . . . . . . . . . . . . . . 35

# 1 Preliminary simulations

We compare the finite sample performance and computational efficiency of GES [Chickering, 2002], GES restricted to an estimated CIG (RGES-CIG) and the order independent version of the PC algorithm [Colombo and Maathuis, 2014].

We choose the high-dimensional settings given in Table 1, and we refer to Section 8.1 of the main text for details on the data generating mechanism.

| Sample size $n$ | 100 | 200 | 300 | 400 |
|---|---|---|---|---|
| Number of variables $p_n$ | 300 | 600 | 1200 | 2400 |
| Expected number of edges $e_n$ | 300 | 840 | 2100 | 4800 |

Table 1: Simulation settings.

We use neighborhood selection with the LASSO of Meinshausen and Bühlmann [2006] for estimating the CIG for RGES-CIG (see Section 8.2 of the main text for details on the choice of tuning parameters). We do not apply GES for the case $p_n = 2400$, due to computational constraints.

As the scoring criterion for GES and RGES-CIG, we use the $\ell_0$ penalized log-likelihood score (see Definition 5.1 of the main text) with a number of choices of the penalty parameter $\lambda_n$. Similarly, we apply PC with a number of choices of its tuning parameter $\alpha_n$ (the significance level for conditional independence tests). We compare the estimation quality with averaged ROC curves, where we average true positive rates and false positive rates for each value of the tuning parameters over 100 iterations (cf. threshold averaging of ROC curves [Fawcett, 2006]).

Figure 1 shows that the estimation performances of GES and RGES-CIG are roughly similar and both of them are significantly better than PC. Figure 2 shows that GES does not scale well to large graphs, but the runtimes of RGES-CIG (see Table 4 in Section 7 for the averaged runtimes of the CIG estimation part) and PC are roughly similar. In summary, our simulations show that RGES-CIG performs about as well as GES in terms of estimation quality, and performs as well as PC in terms of runtime.

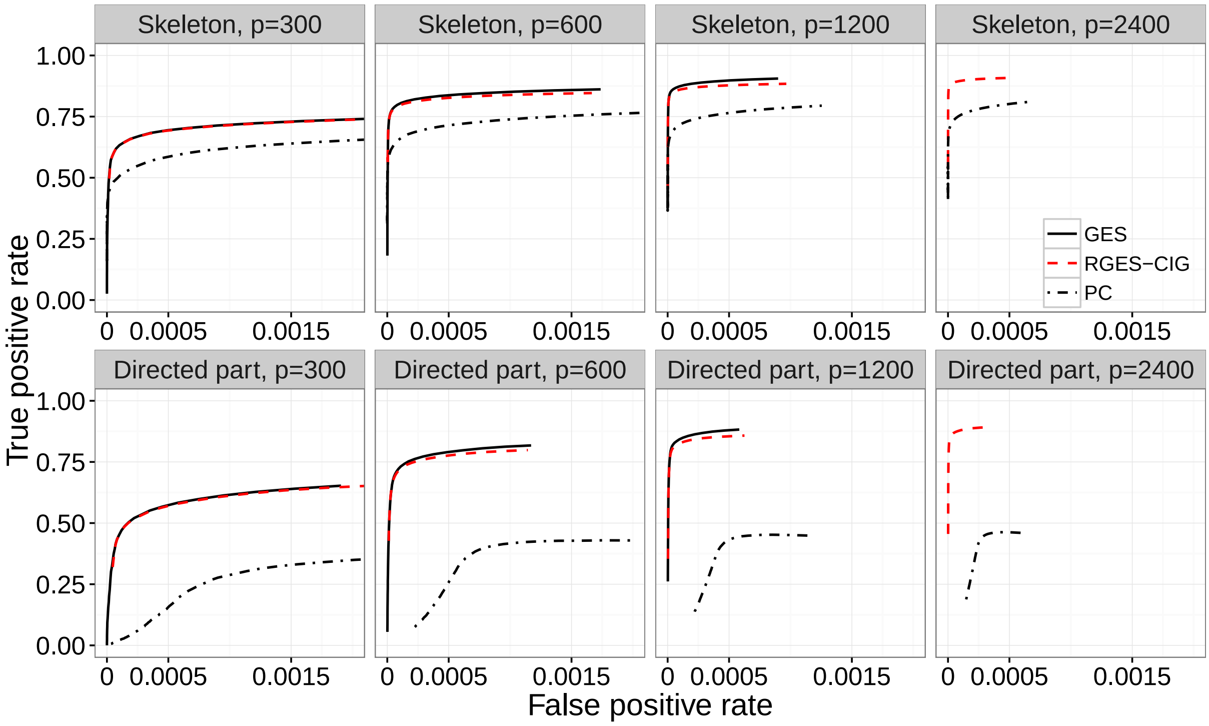


Figure 1: Averaged ROC curves for estimating the skeletons (upper panel) and the directed parts (lower panel) of the underlying CPDAGs with GES, RGES-CIG, and PC.

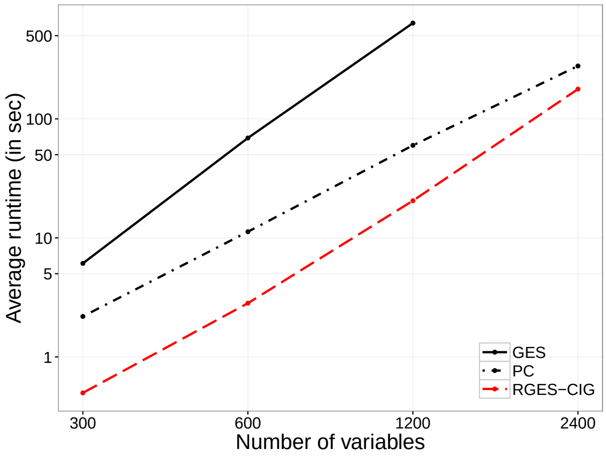


Figure 2: Average runtimes (in seconds) for GES, RGES-CIG, and PC, where the tuning parameters $\alpha_n$ and $\lambda_n$ are chosen to get roughly the right sparsity. The runtimes of RGES-CIG do not include its CIG estimation part (see Table 4 in Section 7).

## 2 Properties of a scoring criterion

**Definition 2.1.** *A scoring criterion $\mathcal{S}$ is* score equivalent *(given a joint distribution) if $\mathcal{S}(\mathcal{H}, \mathcal{D}_n) = \mathcal{S}(\mathcal{H}', \mathcal{D}_n)$ whenever $\mathcal{H}$ and $\mathcal{H}'$ are in the same Markov equivalence class, for any i.i.d. data $\mathcal{D}_n$ from the joint distribution.*

**Definition 2.2.** *A scoring criterion $\mathcal{S}$ is* decomposable *if there is a function $s$ such that for any DAG $\mathcal{H}$ and data $\mathcal{D}_n$ the scoring criterion decomposes as:*

$$\mathcal{S}(\mathcal{H}, \mathcal{D}_n) = \sum_{i=1}^{p} s(X_i, \mathbf{Pa}_{\mathcal{H}}(X_i), \mathcal{D}_n(X_i, \mathbf{Pa}_{\mathcal{H}}(X_i))),$$

*where $\mathcal{D}_n(X_i, \mathbf{Pa}_{\mathcal{H}}(X_i))$ represents the data corresponding to $X_i$ and $\mathbf{Pa}_{\mathcal{H}}(X_i)$.*

**Definition 2.3.** *A scoring criterion $\mathcal{S}$ is* consistent *if the following two properties hold:*

1. *If $\mathcal{H}$ is an independence map (see Definition 2.2 of the main text) of $\mathcal{G}_0$ but $\mathcal{H}'$ is not, then $\lim_{n\to\infty} \mathbb{P}(\mathcal{S}(\mathcal{H}, \mathcal{D}_n) < \mathcal{S}(\mathcal{H}', \mathcal{D}_n)) = 1$, and*
2. *If both $\mathcal{H}$ and $\mathcal{H}'$ are independence maps of $\mathcal{G}_0$ but $\mathcal{H}'$ contains more edges than $\mathcal{H}$, then $\lim_{n\to\infty} \mathbb{P}(\mathcal{S}(\mathcal{H}, \mathcal{D}_n) < \mathcal{S}(\mathcal{H}', \mathcal{D}_n)) = 1$.*

Finally, we define *local consistency* of a scoring criterion. Chickering [2002] showed that any consistent and decomposable score (such as BIC) is locally consistent (see Lemma 7 of Chickering [2002]).

**Definition 2.4.** *(Locally consistent scoring criterion) A scoring criterion $\mathcal{S}$ is* locally consistent *if the following two properties hold, for any pair of nodes $(X_i, X_k)$ in any DAG $\mathcal{H} = (\mathbf{X}, E)$ such that $X_i \in \mathbf{Nd}_{\mathcal{H}}(X_k) \setminus \mathbf{Pa}_{\mathcal{H}}(X_k)$, and the DAG $\mathcal{H}' := (\mathbf{X}, E \cup \{X_i \to X_k\})$:*

1. *If $X_i \not\perp_{\mathcal{G}_0} X_k \mid \mathbf{Pa}_{\mathcal{H}}(X_k)$, then $\lim_{n\to\infty} \mathbb{P}(\mathcal{S}(\mathcal{H}', \mathcal{D}_n) < \mathcal{S}(\mathcal{H}, \mathcal{D}_n)) = 1$, and*
2. *If $X_i \perp_{\mathcal{G}_0} X_k \mid \mathbf{Pa}_{\mathcal{H}}(X_k)$, then $\lim_{n\to\infty} \mathbb{P}(\mathcal{S}(\mathcal{H}', \mathcal{D}_n) > \mathcal{S}(\mathcal{H}, \mathcal{D}_n)) = 1$.*

The first property of Definition 2.4 assures that the score of a DAG $\mathcal{H}$ can be improved (asymptotically) by adding a directed edge if $\mathcal{H}$ is not an independence map of $\mathcal{G}_0$, while the second property assures the converse.

## 3 Pseudocode for GES

Pseudocode of the forward and backward phase of GES is given below. A verbal description of the algorithm can be found in Section 2.4 of the main text.

**Algorithm 3.1** The forward phase of GES

**Input:** A scoring criterion $\mathcal{S}$, the data $\mathcal{D}_n$, an initial CPDAG $\mathcal{C}_{\text{start}}$.
**Output:** A CPDAG

$\mathcal{C}_{\text{new}} \leftarrow \mathcal{C}_{\text{start}}$;
**repeat**
  $\tilde{\mathcal{C}}_n^f \leftarrow \mathcal{C}_{\text{new}}$;
  $\mathfrak{C} \leftarrow$ the set of all CPDAGs $\mathcal{C}$ such that $\mathcal{S}(\mathcal{C}, \mathcal{D}_n) < \mathcal{S}(\tilde{\mathcal{C}}_n^f, \mathcal{D}_n)$, and there exists a DAG in the Markov equivalence class of $\mathcal{C}$ that can be obtained by adding an edge in a DAG in the Markov equivalence class of $\tilde{\mathcal{C}}_n^f$;
  **if** $\mathfrak{C} \neq \emptyset$ **then**
    choose $\mathcal{C}_{\text{new}}$ to be the CPDAG that minimizes the scoring criterion among the CPDAGs in $\mathfrak{C}$;
  **end if**
**until** $\mathfrak{C} = \emptyset$;
**return** $\tilde{\mathcal{C}}_n^f$.

**Algorithm 3.2** The backward phase of GES

**Input:** A scoring criterion $\mathcal{S}$, the data $\mathcal{D}_n$, and the output of the forward phase $\tilde{\mathcal{C}}_n^f$.
**Output:** A CPDAG

$\mathcal{C}_{\text{new}} \leftarrow \tilde{\mathcal{C}}_n^f$;
**repeat**
  $\tilde{\mathcal{C}}_n \leftarrow \mathcal{C}_{\text{new}}$;
  $\mathfrak{C} \leftarrow$ the set of all CPDAGs $\mathcal{C}$ such that $\mathcal{S}(\mathcal{C}, \mathcal{D}_n) \leq \mathcal{S}(\tilde{\mathcal{C}}_n^f, \mathcal{D}_n)$, and there exists a DAG in the Markov equivalence class of $\mathcal{C}$ that can be obtained by deleting an edge in a DAG in the Markov equivalence class of $\tilde{\mathcal{C}}_n$;
  **if** $\mathfrak{C} \neq \emptyset$ **then**
    choose $\mathcal{C}_{\text{new}}$ to be the CPDAG that minimizes the scoring criterion among the CPDAGs in $\mathfrak{C}$;
  **end if**
**until** $\mathfrak{C} = \emptyset$;
**return** $\tilde{\mathcal{C}}_n$.

# 4 Additional details for Example 1 of the main text

## 4.1 Search paths

Figure 3 shows the search paths of GES, RGES-CIG and RGES-skeleton for Example 1 of the main text, where each transition from a CPDAG to another CPDAG represents a single step of the forward or the backward phase. Note that the search paths of RGES-CIG

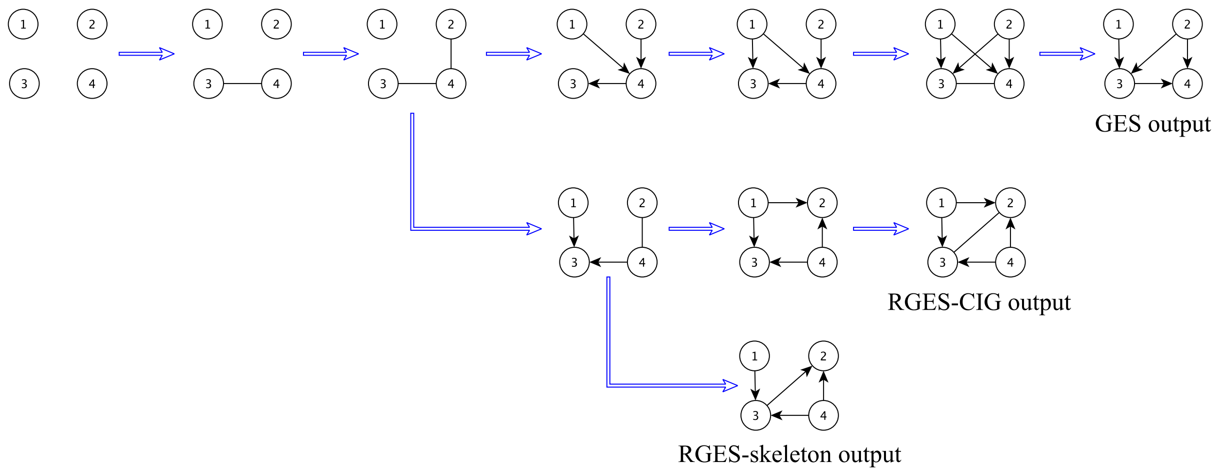


Figure 3: Search paths of GES, RGES-CIG and RGES-skeleton, where node $i$ represents variable $X_i$.

and RGES-skeleton only consist of their forward phases, whereas the last step in the search path of GES corresponds to its backward phase.

The output of GES is the same as the true CPDAG. We see that while adding the edge $1 \to 4$ in the third step, GES wrongly orients the edge $3 \leftarrow 4$. GES eventually manages to recover from this "wrong move" with the last two steps. First, it adds a shield to the unshielded triple $3 \leftarrow 4 \leftarrow 2$ and consequently changes $3 \leftarrow 4$ into $3 - 4$. Next, it correctly orients $3 - 4$ as $3 \to 4$ while deleting the edge $1 \to 4$.

The first two steps of RGES-CIG and GES are identical. In the third step, RGES-CIG cannot add the edge $1 \to 4$ as nodes 1 and 4 are non-adjacent in the CIG (Figure 1b of the main text). It adds the edge $1 \to 3$ instead and also wrongly orients the edge between nodes 3 and 4 by creating the v-structure $1 \to 3 \leftarrow 4$. In contrast to GES, RGES-CIG cannot reorient the edge $3 \leftarrow 4$, since the shield of the v-structure $1 \to 3 \leftarrow 4$ is not allowed in RGES-CIG. RGES-skeleton encounters the same problem.

In summary, we see that naive restrictions on the search space of GES can interrupt its self-recovering property and consequently, lead to inconsistency.

## 4.2 Computation of large sample limits

Let $\mathcal{H} = (\mathbf{X}, E_{\mathcal{H}})$ be any DAG with vertex set $\mathbf{X}$ and edge set $E_{\mathcal{H}}$ and let $\mathcal{D}_n$ denote the data, consisting of $n$ i.i.d. observations of $\mathbf{X}$. Let $|E_{\mathcal{H}}|$ denote the number of edges of $\mathcal{H}$. The BIC criterion is given by

$$\mathcal{S}_n(\mathcal{H}, \mathcal{D}_n) = -2 \sum_{i=1}^{p} \log \Big( L(\hat{\boldsymbol{\theta}}_i(\mathcal{H}), \mathcal{D}_n(X_i) | \mathcal{D}_n(\mathbf{Pa}_{\mathcal{H}}(X_i))) \Big) + |E_{\mathcal{H}}| \log(n),$$

where $L(\boldsymbol{\theta}_i(\mathcal{H}), \mathcal{D}_n(X_i)|\mathcal{D}_n(\mathbf{Pa}_{\mathcal{H}}(X_i)))$ is the likelihood function that corresponds to the conditional density of $X_i$ given $\mathbf{Pa}_{\mathcal{H}}(X_i)$ under parameter $\boldsymbol{\theta}_i(\mathcal{H})$, and

$$\hat{\boldsymbol{\theta}}_i(\mathcal{H}) = \underset{\boldsymbol{\theta}_i(\mathcal{H})}{\operatorname{argmax}} \ \log\Big(L(\boldsymbol{\theta}_i(\mathcal{H}), \mathcal{D}_n(X_i)|\mathcal{D}_n(\mathbf{Pa}_{\mathcal{H}}(X_i)))\Big)$$

is the maximum likelihood estimate (MLE) of the parameter vector $\boldsymbol{\theta}_i(\mathcal{H})$.

If $\mathbf{X}$ is multivariate Gaussian, then $\boldsymbol{\theta}_i(\mathcal{H})$ is given by the conditional mean and the conditional variance of $X_i \mid \mathbf{Pa}_{\mathcal{H}}(X_i)$. Specifically, $\boldsymbol{\theta}_i(\mathcal{H}) = (\mu_i, \boldsymbol{\beta}_i(\mathcal{H})^T, \sigma_i(\mathcal{H}))^T$, where $\mathrm{E}[X_i \mid \mathbf{Pa}_{\mathcal{H}}(X_i)] = \mu_i + \boldsymbol{\beta}_i(\mathcal{H})^T\mathbf{Pa}_{\mathcal{H}}(X_i)$ and $\sigma_i(\mathcal{H})^2 = \mathrm{Var}[X_i \mid \mathbf{Pa}_{\mathcal{H}}(X_i)]$. Moreover, it can be shown (see the proof of Lemma 5.1 of the main text) that

$$\frac{1}{n}\mathcal{S}_n(\mathcal{H}, \mathcal{D}_n) = \sum_{i=1}^{p} \log(2\pi\hat{\sigma}_i(\mathcal{H})^2) + p + \frac{\log(n)}{n}|E_{\mathcal{H}}|,$$

where $\hat{\sigma}_i(\mathcal{H})^2$ is the variance of the residuals of the regression of $X_i$ on $\mathbf{Pa}_{\mathcal{H}}(X_i)$ based on the data $\mathcal{D}_n$. Therefore, $\mathcal{S}_n(\mathcal{H}, \mathcal{D}_n)/n$ converges to $\mathcal{S}^*(\mathcal{H}, \Sigma_0) = \sum_{i=1}^{p} \log(2\pi\sigma_i(\mathcal{H})^2) + p$ almost surely. Thus the large sample limit outputs of (hybrid versions of) GES with the BIC criterion are equal to the outputs of (hybrid versions of) GES with the scoring criterion $\mathcal{S}^*(\mathcal{H}, \Sigma_0)$.

When implementing (hybrid versions of) GES with scoring criterion $\mathcal{S}^*$, a (theoretically) zero score difference can be nonzero on a computer due to numerical errors. This can be resolved by thresholding score differences at a tolerance level $\eta$, which is equivalent to using the penalized scoring criterion $\mathcal{S}^*_\eta(\mathcal{H}, \Sigma_0) = \mathcal{S}^*(\mathcal{H}, \Sigma_0) + \eta|E_{\mathcal{H}}|$.

## 4.3 Large sample limit outputs of hill-climbing DAG search and its hybrid versions

Given a scoring criterion, hill-climbing DAG search starts with an initial DAG and aims to greedily optimize the score function on the space of DAGs, by adding, deleting or turning exactly one edge at every step until the score can no longer be improved. At every step, among all the possible single edge moves that decrease the score, it selects the one that minimizes the score.

Note that edge additions in (hybrid versions of) hill-climbing DAG search are, in general, not uniquely defined. At some steps, the algorithm may need to select an orientation of an edge addition, while both orientations lead to the same score improvement (due to Markov equivalence of the resulting DAGs). Although the final output, in general, depends on these choices, they are often made arbitrarily. We show that (restricted-versions) of hill-climbing DAG search are inconsistent, meaning that they are inconsistent for at least one set of such choices. In particular, if adding $X_i \rightarrow X_j$ and $X_j \rightarrow X_i$ lead to the same score, we choose $X_i \rightarrow X_j$ if and only if $i < j$.

The large sample limit outputs of hill-climbing DAG search and its hybrid versions are given in Figure 4, and all of them are different from $\mathcal{G}_0 = \mathrm{CPDAG}(\mathcal{G}_0)$ (see Figure 1(a) of the main text). We initialized all algorithms by the empty graph and determined the large sample limit outputs using the scoring criterion $\mathcal{S}^*$ defined in Section 4.2.

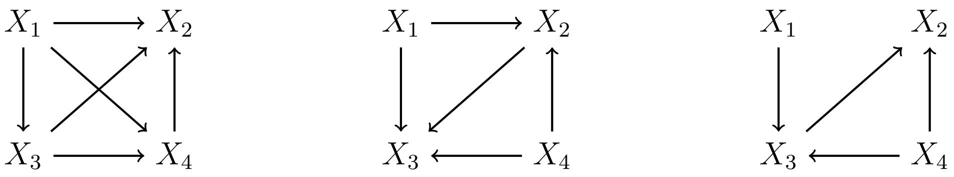


(a) (b) (c)

Figure 4: The DAGs in (a), (b) and (c) are the large sample limit outputs of hill-climbing DAG search, hill-climbing DAG search restricted to the CIG and hill-climbing DAG search restricted to the CPDAG-skeleton, respectively.

# 5 Empirical verification of Assumption (A5) of the main text

We choose the same high-dimensional settings as in Section 8.1 of the main text and Section 1: $(p_n, e_n) = (300, 300)$, $(600, 840)$, $(1200, 2100)$ and $(2400, 4800)$. We refer to Section 8.1 of the main text for more details.

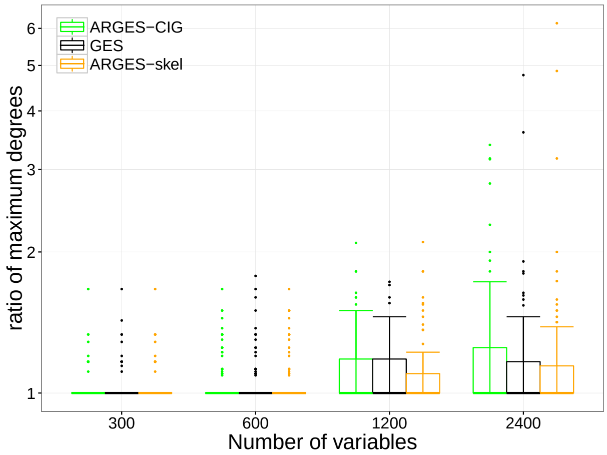


Figure 5: Boxplots for the ratio of the maximum degree of the output of the oracle forward phase of (AR)GES and the maximum degree of the corresponding true CPDAG.

Figure 5 shows that the ratio of the maximum degree of the output of the oracle forward phase of GES and the maximum degree of the corresponding true CPDAG slowly increases as the number of variables $p_n$ increases, and the ratios are roughly bounded by 2 (except for few outliers) with the median equal to 1 for all four values of $p_n$. Note that this ratio corresponds to $K_n$ in Assumption (A5) of the main text. We initialized all algorithms by the empty graph and we used the oracle scoring criterion $\mathcal{S}^*_{\lambda_n}$ (see Definition 5.2 of the main text) with $\lambda_n = 10^{-5}$.

# 6 Inclusion of a turning phase in (AR)GES

It has been shown empirically that the inclusion of a so-called turning phase in GES can lead to better estimation performance [Hauser and Bühlmann, 2012]. In the turning phase, which starts with the output of the backward phase, the algorithm changes the orientation of exactly one directed edge at each step. It selects the optimal move at each step according to the scoring criterion and stops when the current score can no longer be improved by turning a directed edge. One may obtain even better estimation performance by iterating over all three phases (forward, backward and turning), until some pre-defined convergence criterion is satisfied, a pragmatic approach that is implemented in the R-package **pcalg** [Kalisch et al., 2012]. These modifications can also be implemented in ARGES, and we included the turning phase and an iteration over the three phases for (AR)GES in all simulations. We note that these modifications do not affect our theoretical results.

# 7 Effect of the tuning parameter $\gamma_n$ on the performance ARGES-CIG

We investigate the effect of the tuning parameter $\gamma_n$ on the performance of ARGES-CIG with the same high-dimensional settings as in Section 8.1 of the main text for $p_n = 300$, 600, and 1200 (see Table 2). For each setting, we choose six different values of $\gamma_n$ that are given by Table 2.

| $n$ | $p_n$ | $e_n$ | $\gamma_n$ | | | | | |
|---|---|---|---|---|---|---|---|---|
| 100 | 300 | 300 | 0.10 | 0.12 | 0.14 | 0.16 | 0.18 | 0.20 |
| 200 | 600 | 840 | 0.08 | 0.10 | 0.12 | 0.14 | 0.16 | 0.18 |
| 300 | 1200 | 2100 | 0.06 | 0.08 | 0.10 | 0.12 | 0.14 | 0.16 |

Table 2: Choice of the tuning parameter $\gamma_n$ for estimating CIG for ARGES-CIG.

As the scoring criterion for GES and ARGES-CIG, we use the $\ell_0$-penalized likelihood score (see Definition 5.1 of the main text) with a number of choices of the penalty parameter $\lambda_n$. Then we compare the estimation quality of GES and ARGES-CIG with averaged ROC curves, where we average true positive rates and false positive rates for each value of the tuning parameters over $r$ iterations (cf. threshold averaging of ROC curves [Fawcett, 2006]).

Figure 6 shows that the performance of ARGES-CIG is not very sensitive to the choice of $\gamma_n$, and that the ROC curve of ARGES-CIG slowly improves and eventually converges to the ROC curve of GES as $\gamma_n$ decreases. Recall that smaller values of $\gamma_n$ lead to denser estimates of the CIG and thus increased runtimes of ARGES-CIG. Note that ARGES-CIG based on the complete undirected graph is the same as GES and hence the runtime of GES is roughly an upper bound of the runtime of the GES part of ARGES-CIG. However, Table 3 shows that the runtime of ARGES-CIG is much better than GES as long as $\gamma_n$ is not too small.

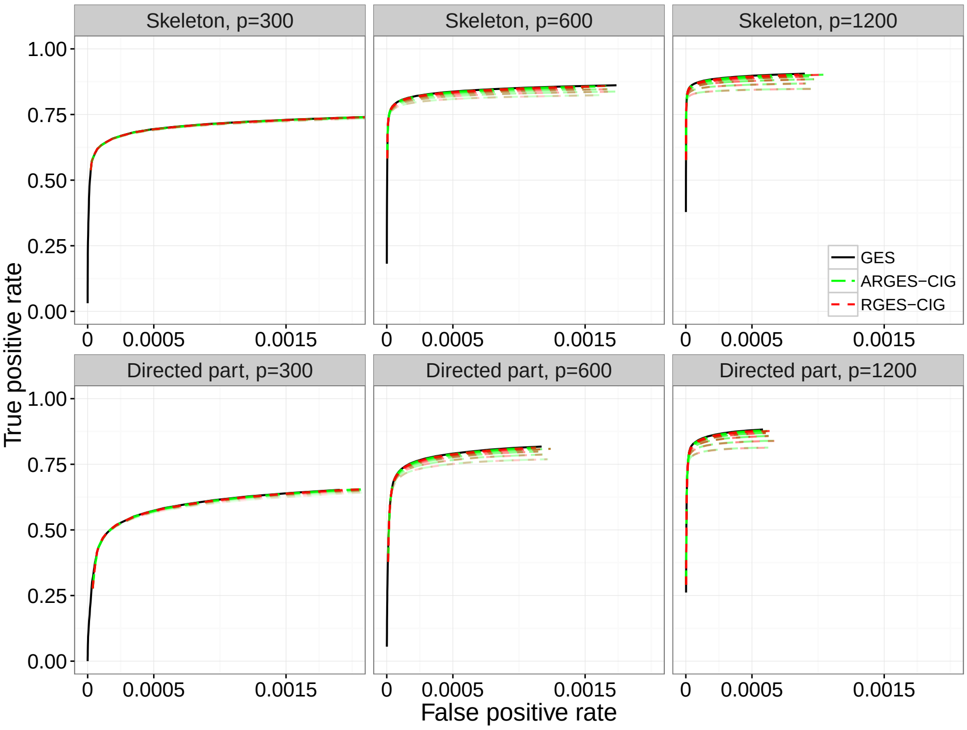


Figure 6: Averaged ROC curves for estimating the skeletons (left panel) and the directed parts (right panel) of the underlying CPDAGs with ARGES-CIG, RGES-CIG and GES. Here ROC curves for (A)RGES-CIG with higher values of $\gamma_n$ (see Table 2) are plotted with lighter colors.

| Method | $p_n$ | $\gamma_n$ | $\frac{2\|E_{\hat{\mathcal{I}}_n}\|}{p_n(p_n-1)}$ | $\frac{\|E_{\hat{\mathcal{I}}_n}\|}{\|E_{\mathcal{I}_{n0}}\|}$ | Runtime (CIG part) | Runtime (GES part) |
|---|---|---|---|---|---|---|
| ARGES-CIG | 300 | 0.20 | 0.027 (0.0008) | 2.5 (0.26) | 0.6 (0.03) | 0.7 (0.3) |
| ARGES-CIG | 300 | 0.16 | 0.054 (0.0016) | 5.0 (0.53) | 0.6 (0.03) | 0.6 (0.3) |
| ARGES-CIG | 300 | 0.10 | 0.136 (0.0030) | 12.6 (1.33) | 0.7 (0.04) | 0.6 (0.3) |
| GES | 300 | – | – | – | – | 6.1 (1.0) |
| ARGES-CIG | 600 | 0.18 | 0.008 (0.0002) | 0.9 (0.05) | 0.7 (0.11) | 4.4 (2.6) |
| ARGES-CIG | 600 | 0.14 | 0.022 (0.0006) | 2.4 (0.16) | 0.8 (0.11) | 4.6 (2.7) |
| ARGES-CIG | 600 | 0.08 | 0.095 (0.0022) | 10.7 (0.70) | 0.8 (0.11) | 4.5 (2.7) |
| GES | 600 | – | – | – | – | 69 (10) |
| ARGES-CIG | 1200 | 0.16 | 0.004 (0.0001) | 0.7 (0.03) | 1.7 (0.95) | 37 (23) |
| ARGES-CIG | 1200 | 0.12 | 0.013 (0.0003) | 2.0 (0.10) | 1.7 (0.94) | 35 (22) |
| ARGES-CIG | 1200 | 0.06 | 0.084 (0.0017) | 13.4 (0.68) | 1.8 (0.97) | 38 (24) |
| GES | 1200 | – | – | – | – | 638 (85) |

Table 3: Average density (the fourth column) of the estimated CIGs $\hat{\mathcal{I}}_n$, average of the ratios of the density of $\hat{\mathcal{I}}_n$ and the density of the true CIG $\mathcal{I}_{n0}$ (the fifth column), the average runtime for estimating $\hat{\mathcal{I}}_n$ (the sixth column), and average runtimes of the GES part of the algorithms (the last column). The numbers in brackets are the corresponding standard deviations.

# 8 CIG and CPDAG-skeleton estimation results corresponding to Section 8.3 of the main text

Table 4 compares the average runtimes of neighborhood selection and MMPC, the average densities of their outputs $\hat{\mathcal{I}}_n$ and $\hat{\mathcal{U}}_n$, and their average true positive rates (TPR). The density of a graph with $p$ vertices and $|E|$ edges is $|E|/\binom{p}{2}$. We see that the estimated CPDAG-skeletons are much sparser than the estimated CIGs, while the average runtimes of MMPC are much larger than the average runtimes of neighborhood selection.

| Number of variables ($p_n$) | 300 | 600 | 1200 | 2400 |
|---|---|---|---|---|
| Expected number of edges ($e_n$) | 300 | 840 | 2100 | 4800 |
| Runtime of neighborhood selection | 0.6 | 0.8 | 1.7 | 5 |
| Density of $\hat{\mathcal{I}}_n$ | 0.054 | 0.022 | 0.013 | 0.011 |
| TPR of $\hat{\mathcal{I}}_n$ | 0.86 | 0.89 | 0.90 | 0.93 |
| Runtime of MMPC | 40 | 545 | 2319 | 3656 |
| Density of $\hat{\mathcal{U}}_n$ | 0.015 | 0.009 | 0.004 | 0.002 |
| TPR of $\hat{\mathcal{U}}_n$ | 0.72 | 0.79 | 0.80 | 0.81 |

Table 4: Average runtimes (in seconds) of neighborhood selection and MMPC, and average densities and true positive rates of $\hat{\mathcal{I}}_n$ and $\hat{\mathcal{U}}_n$, $p_n = 300$, 600, 1200 and 2400.

# 9 Proofs

## 9.1 Proof of Theorem 4.1 of the main text

We will use the following additional graph terminology in this subsection. A subpath of $\pi_{\mathcal{A}}(X_i, X_{i+1}, \ldots, X_{i+q})$ is a path of the form $\pi_{\mathcal{A}}(X_j, X_{j+1}, \ldots, X_{j+s})$, for some $j$ and $s$ satisfying $i \leq j \leq j+s \leq i+q$. A set $\mathbf{S}$ *intersects* a path $\pi_{\mathcal{A}}(X_i, \ldots, X_k)$ if $\mathbf{S} \cap \{X_i, \ldots, X_k\}$ is non-empty. If $\mathbf{S} = \{X_r\}$ intersects a path $\pi_{\mathcal{A}}(X_i, \ldots, X_k)$, we will simply say that $X_r$ intersects the path.

As discussed in the main text, the "if part" of Theorem 4.1 of the main text follows from Proposition 27 and Lemma 28 of Chickering [2002]. Thus we only prove the other direction. To this end, it suffices to show that if a DAG $\mathcal{H}$ is not an independence map of $\mathcal{G}$ and the first two conditions of Theorem 4.1 of the main text do not hold for $\mathcal{H}$, then the third condition must hold. We state this as the following lemma.

**Lemma 9.1.** *If a DAG $\mathcal{H}$ is not an independence map of $\mathcal{G}$, and*

**(a1)** skeleton($\mathcal{G}$) $\subseteq$ skeleton($\mathcal{H}$) *and*

**(a2)** *for all triples of nodes $\{X_i, X_j, X_k\}$ such that $\pi_{\mathcal{G}}(X_i, X_j, X_k)$ is a v-structure and $\pi_{\mathcal{H}}(X_i, X_j, X_k)$ is a non-collider path, we have $X_i \in \mathbf{Adj}_{\mathcal{H}}(X_k)$,*

*then there exists a triple of nodes* $\{X_i, X_j, X_k\}$ *such that* $\pi_{\mathcal{H}}(X_i, X_j, X_k)$ *is a v-structure,* $X_i \not\perp_{\mathcal{G}} X_k \mid \mathbf{Pa}_{\mathcal{H}}(X_k)$ *and* $X_i \in \mathbf{Nd}_{\mathcal{H}}(X_k)$*.*

The proof of Lemma 9.1 is quite lengthy and we first present the main idea by considering two special cases. In order to define these special cases, we recall that the set of all d-separations in $\mathcal{H}$ is characterized by $\{X_r \perp_{\mathcal{H}} \mathbf{Nd}_{\mathcal{H}}(X_r) \setminus \mathbf{Pa}_{\mathcal{H}}(X_r) \mid \mathbf{Pa}_{\mathcal{H}}(X_r) : r = 1, \ldots, p\}$ [Verma and Pearl, 1990]. Therefore, $\mathcal{H}$ is not an independence map of $\mathcal{G}$ implies that there exists a pair of nodes $\{X_i, X_k\}$ such that $X_i \in \mathbf{Nd}_{\mathcal{H}}(X_k) \setminus \mathbf{Pa}_{\mathcal{H}}(X_k)$ and $X_i \not\perp_{\mathcal{G}} X_k \mid \mathbf{Pa}_{\mathcal{H}}(X_k)$ meaning that there exists a path $\pi_{\mathcal{G}}(X_i, \ldots, X_k)$ that is open given $\mathbf{Pa}_{\mathcal{H}}(X_k)$.

The first special case is that the path $\pi_{\mathcal{G}}(X_i, \ldots, X_k)$ consists of three nodes $(X_i, X_j, X_k)$, for some $X_j$. We then prove Lemma 9.1 by showing that $(X_i, X_j, X_k)$ is a v-structure in $\mathcal{H}$.

**Lemma 9.2.** *Suppose* $\mathcal{H}$ *and* $\mathcal{G}$ *are two DAGs that satisfy (a1) and (a2) of Lemma 9.1. If there exists a triple of nodes* $\{X_i, X_j, X_k\}$ *such that* $X_i \in \mathbf{Nd}_{\mathcal{H}}(X_k) \setminus \mathbf{Pa}_{\mathcal{H}}(X_k)$ *and* $(X_i, X_j, X_k)$ *is path in* $\mathcal{G}$ *such that* $\pi_{\mathcal{G}}(X_i, X_j, X_k)$ *is open given* $\mathbf{Pa}_{\mathcal{H}}(X_k)$*, then* $(X_i, X_j, X_k)$ *is a v-structure in* $\mathcal{H}$*.*

*Proof.* By (a1), the path $\pi_{\mathcal{H}}(X_i, X_j, X_k)$ exists in $\mathcal{H}$. Suppose $\pi_{\mathcal{H}}(X_i, X_j, X_k)$ is not a v-structure. Then $\pi_{\mathcal{H}}(X_i, X_j, X_k)$ must be a non-collider path, since $X_i$ and $X_k$ are not adjacent in $\mathcal{H}$. Further, since $X_i \in \mathbf{Nd}_{\mathcal{H}}(X_k)$, $\pi_{\mathcal{H}}(X_i, X_j, X_k)$ must be either $X_i \rightarrow X_j \rightarrow X_k$ or $X_i \leftarrow X_j \rightarrow X_k$ implying that $X_j \in \mathbf{Pa}_{\mathcal{H}}(X_k)$. Now $X_j \in \mathbf{Pa}_{\mathcal{H}}(X_k)$ and $\pi_{\mathcal{G}}(X_i, X_j, X_k)$ being open given $\mathbf{Pa}_{\mathcal{H}}(X_k)$ imply that $X_j$ is a collider on the path $\pi_{\mathcal{G}}(X_i, X_j, X_k)$. In fact, $\pi_{\mathcal{G}}(X_i, X_j, X_k)$ is a v-structure, since (a1) and the fact that $X_i$ and $X_k$ are not adjacent in $\mathcal{H}$, implies that $X_i$ and $X_k$ are not adjacent in $\mathcal{G}$. This contradicts (a2). Hence, $\pi_{\mathcal{H}}(X_i, X_j, X_k)$ must be a v-structure. □

The second special case is that $\pi_{\mathcal{G}}(X_i, \ldots, X_k)$ is a non-collider path. We then prove Lemma 9.1 by showing that there exists a triple of nodes $\{X_{i'}, X_{j'}, X_{k'}\}$ such that $X_{i'} \in \mathbf{Nd}_{\mathcal{H}}(X_{k'}) \setminus \mathbf{Pa}_{\mathcal{H}}(X_{k'})$, $\pi_{\mathcal{H}}(X_{i'}, X_{j'}, X_{k'})$ is a v-structure and $X_{i'} \not\perp_{\mathcal{G}} X_{k'} \mid \mathbf{Pa}_{\mathcal{H}}(X_{k'})$.

**Lemma 9.3.** *Suppose* $\mathcal{H}$ *and* $\mathcal{G}$ *are two DAGs that satisfy (a1) of Lemma 9.1. If there exists a pair of nodes* $\{X_i, X_k\}$ *and a non-collider path* $\pi_{\mathcal{G}}(X_i, \ldots, X_k)$ *such that* $X_i \in \mathbf{Nd}_{\mathcal{H}}(X_k) \setminus \mathbf{Pa}_{\mathcal{H}}(X_k)$ *and* $\pi_{\mathcal{G}}(X_i, \ldots, X_k)$ *is open given* $\mathbf{Pa}_{\mathcal{H}}(X_k)$*, then there exists a triple of nodes* $\{X_{i'}, X_{j'}, X_{k'}\}$ *such that* $X_{i'} \in \mathbf{Nd}_{\mathcal{H}}(X_{k'}) \setminus \mathbf{Pa}_{\mathcal{H}}(X_{k'})$*,* $\pi_{\mathcal{H}}(X_{i'}, X_{j'}, X_{k'})$ *is a v-structure and* $X_{i'} \not\perp_{\mathcal{G}} X_{k'} \mid \mathbf{Pa}_{\mathcal{H}}(X_{k'})$*.*

*Proof.* By (a1), $\pi_{\mathcal{H}}(X_i, \ldots, X_k)$ exists. Since the non-collider path $\pi_{\mathcal{G}}(X_i, \ldots, X_k)$ is open given $\mathbf{Pa}_{\mathcal{H}}(X_k)$, $\mathbf{Pa}_{\mathcal{H}}(X_k)$ does not intersect $\pi_{\mathcal{G}}(X_i, \ldots, X_k)$. Hence, every path in $\mathcal{H}$ between $X_i$ and $X_k$ consisting of a subsequence of the nodes on $\pi_{\mathcal{H}}(X_i, \ldots, X_k)$ must contain a collider (as $X_i \perp_{\mathcal{H}} X_k \mid \mathbf{Pa}_{\mathcal{H}}(X_k)$). Therefore, by Lemma 9.4 below, there exists a triple of nodes $\{X_{i'}, X_{j'}, X_{k'}\}$ on the path $\pi_{\mathcal{H}}(X_i, \ldots, X_k)$ such that

1. $\pi_{\mathcal{H}}(X_{i'}, X_{j'}, X_{k'})$ is a v-structure, and

2. for all non-endpoint nodes $X_r$ on the subpath $\pi_{\mathcal{H}}(X_{i'}, \ldots, X_{k'})$ of $\pi_{\mathcal{H}}(X_i, \ldots, X_k)$, $X_r \in \mathbf{De}_{\mathcal{H}}(X_{i'}) \cap \mathbf{De}_{\mathcal{H}}(X_{k'})$.

Without loss of generality, we assume that $X_{i'} \in \mathbf{Nd}_{\mathcal{H}}(X_{k'})$. Thus it remains to show that $X_{i'} \not\perp_{\mathcal{G}} X_{k'} \mid \mathbf{Pa}_{\mathcal{H}}(X_{k'})$. Note that $\mathbf{Pa}_{\mathcal{H}}(X_{k'})$ does not intersect $\pi_{\mathcal{H}}(X_{i'}, \ldots, X_{k'})$ as all non-endpoint nodes on $\pi_{\mathcal{H}}(X_{i'}, \ldots, X_{k'})$ are descendants of $X_{k'}$. Thus $\mathbf{Pa}_{\mathcal{H}}(X_{k'})$ does not intersect the corresponding subpath $\pi_{\mathcal{G}}(X_{i'}, \ldots, X_{k'})$ of the non-collider path $\pi_{\mathcal{G}}(X_i, \ldots, X_k)$. Therefore, the non-collider path $\pi_{\mathcal{G}}(X_{i'}, \ldots, X_{k'})$ is open given $\mathbf{Pa}_{\mathcal{H}}(X_{k'})$ and hence $X_{i'} \not\perp_{\mathcal{G}} X_{k'} \mid \mathbf{Pa}_{\mathcal{H}}(X_{k'})$. □

**Lemma 9.4.** *Let $\mathcal{H}$ be a directed graph and let $\pi_{\mathcal{H}}(X_i, \ldots, X_k)$ be a path in $\mathcal{H}$ containing at least three nodes. If (i) $X_i$ and $X_k$ are non-adjacent in $\mathcal{H}$ and (ii) every path in $\mathcal{H}$ between $X_i$ and $X_k$ consisting of a subsequence of the nodes on $\pi_{\mathcal{H}}(X_i, \ldots, X_k)$ contains a collider, then there exists a triple of nodes $\{X_{i'}, X_{j'}, X_{k'}\}$ on the path $\pi_{\mathcal{H}}(X_i, \ldots, X_k)$ such that*

*1. $\pi_{\mathcal{H}}(X_{i'}, X_{j'}, X_{k'})$ is a v-structure, and*

*2. for all non-endpoint nodes $X_r$ on the subpath $\pi_{\mathcal{H}}(X_{i'}, \ldots, X_{k'})$ of $\pi_{\mathcal{H}}(X_i, \ldots, X_k)$, $X_r \in \mathbf{De}_{\mathcal{H}}(X_{i'}) \cap \mathbf{De}_{\mathcal{H}}(X_{k'})$.*

*Proof.* Let $\pi_{\mathcal{H}}(X_i, \ldots, X_k)$ be a path containing at least three nodes satisfying conditions (i) and (ii) of Lemma 9.4. We prove the result by induction on the number of nodes in $\pi_{\mathcal{H}}(X_i, \ldots, X_k)$. For a path $\pi_{\mathcal{H}}(X_i, X_j, X_k)$ containing three nodes, the conditions that $X_i$ and $X_k$ are non-adjacent in $\mathcal{H}$ and $\pi_{\mathcal{H}}(X_i, X_j, X_k)$ is a collider path, imply that the result holds with $(i', j', k') = (i, j, k)$.

Now we assume that $\pi_{\mathcal{H}}(X_i, \ldots, X_k)$ contains $q$ nodes, with $q > 3$ and that the result holds for all paths containing $q - 1$ nodes. Let $X_s$ be a collider on $\pi_{\mathcal{H}}(X_i, \ldots, X_k)$, and let $X_{s^-}$ and $X_{s^+}$ be the nodes on $\pi_{\mathcal{H}}(X_i, \ldots, X_k)$ that precede and succeed $X_s$, respectively. If $X_{s^-}$ and $X_{s^+}$ are non-adjacent in $\mathcal{H}$, then the result holds with $(i', j', k') = (s^-, s, s^+)$. If $X_{s^-}$ and $X_{s^+}$ are adjacent in $\mathcal{H}$, we consider the path $\pi_{\mathcal{H}}(X_i, \ldots, X_{s^-}, X_{s^+}, \ldots, X_k)$, containing $q - 1$ nodes. By the induction hypothesis, there exists a triple of nodes $\{X_{i'}, X_{j'}, X_{k'}\}$ on the path $\pi_{\mathcal{H}}(X_i, \ldots, X_{s^-}, X_{s^+}, \ldots, X_k)$ such that $\pi_{\mathcal{H}}(X_{i'}, X_{j'}, X_{k'})$ is a v-structure and for all non-endpoint nodes $X_r$ on the subpath $\pi_{\mathcal{H}}(X_{i'}, \ldots, X_{k'})$ of $\pi_{\mathcal{H}}(X_i, \ldots, X_{s^-}, X_{s^+}, \ldots, X_k)$, $X_r \in \mathbf{De}_{\mathcal{H}}(X_{i'}) \cap \mathbf{De}_{\mathcal{H}}(X_{k'})$.

If $\pi_{\mathcal{H}}(X_{i'}, \ldots, X_{k'})$ is a subpath of $\pi_{\mathcal{H}}(X_i, \ldots, X_{s^-})$ or a subpath of $\pi_{\mathcal{H}}(X_{s^+}, \ldots, X_k)$, then we are done. Otherwise, both $X_{s^-}$ and $X_{s^+}$ intersect $\pi_{\mathcal{H}}(X_{i'}, \ldots, X_{k'})$, and in this case we need to show that $X_s \in \mathbf{De}_{\mathcal{H}}(X_{i'}) \cap \mathbf{De}_{\mathcal{H}}(X_{k'})$. If $s^- = i'$ or $s^+ = i'$, then $X_s \in \mathbf{De}_{\mathcal{H}}(X_{i'})$ trivially holds. If $s^-, s^+ \neq i'$ and both $X_{s^-}$ and $X_{s^+}$ intersect $\pi_{\mathcal{H}}(X_{i'}, \ldots, X_{k'})$, then at least one of $X_{s^-}$ and $X_{s^+}$ must be a non-endpoint node on $\pi_{\mathcal{H}}(X_{i'}, \ldots, X_{k'})$ and hence a descendant of $X_{i'}$. This implies $X_s \in \mathbf{De}_{\mathcal{H}}(X_{i'})$, since $\{X_{s^-}, X_{s^+}\} \subseteq \mathbf{Pa}_{\mathcal{H}}(X_s)$. Similar arguments with the cases $\{s^-, s^+\} \cap \{k'\} \neq \emptyset$ and $\{s^-, s^+\} \cap \{k'\} = \emptyset$ imply $X_s \in \mathbf{De}_{\mathcal{H}}(X_{k'})$. □

**Proof of Lemma 9.1.** Let $\mathcal{H}$ be a DAG that is not an independence map of $\mathcal{G}$, satisfying (a1) and (a2). This implies that there exist a pair of nodes $\{X_i, X_k\}$ and a path $\pi_{\mathcal{G}}(X_i, \dots, X_k)$ such that $X_i \in \mathbf{Nd}_{\mathcal{H}}(X_k) \setminus \mathbf{Pa}_{\mathcal{H}}(X_k)$ and $\pi_{\mathcal{G}}(X_i, \dots, X_k)$ is open given $\mathbf{Pa}_{\mathcal{H}}(X_k)$. Among all such triples of two nodes and a path between them, i.e., $(X_i, X_k, \pi_{\mathcal{G}}(X_i, \dots, X_k))$, we first consider those triples for which the path contains the minimum number of colliders and we denote that minimum number by $m$. Next, among all such triples where the path contains exactly $m$ colliders, we choose a triple that has a shortest path. Let $(X_1, X_q, \pi_{\mathcal{G}}(X_1, X_2, \dots, X_q))$ be the chosen triple.

For ease of reference, we first list some useful properties that follow from (a1), (a2) and the definition of the triple $(X_1, X_q, \pi_{\mathcal{G}}(X_1, X_2, \dots, X_q))$.

**(p1)** The path $\pi_{\mathcal{H}}(X_1, X_2, \dots, X_q)$ exists;

**(p2)** $X_1 \in \mathbf{Nd}_{\mathcal{H}}(X_q) \setminus \mathbf{Pa}_{\mathcal{H}}(X_q)$ and hence $X_1 \perp_{\mathcal{H}} X_q \mid \mathbf{Pa}_{\mathcal{H}}(X_q)$;

**(p3)** The path $\pi_{\mathcal{G}}(X_1, X_2, \dots, X_q)$ is open given $\mathbf{Pa}_{\mathcal{H}}(X_q)$;

**(p4)** For all $s \in \{2, \dots, q-1\}$: if $X_s \in \mathbf{Pa}_{\mathcal{H}}(X_q)$, then $X_s$ is a collider on the path $\pi_{\mathcal{G}}(X_1, X_2, \dots, X_q)$;

**(p5)** For all $r \in \{2, \dots, q-1\}$: if $X_r \notin \mathbf{Pa}_{\mathcal{H}}(X_q)$, then $X_r \in \mathbf{De}_{\mathcal{H}}(X_q)$;

**(p6)** For all $s \in \{2, \dots, q-1\}$: if $X_s \in \mathbf{Pa}_{\mathcal{H}}(X_q)$, then $X_{s-1} \in \mathbf{Adj}_{\mathcal{H}}(X_{s+1})$.

Property (p1) follows from (a1). Properties (p2) and (p3) follow from the definition of the triple $(X_1, X_q, \pi_{\mathcal{G}}(X_1, X_2, \dots, X_q))$. Property (p4) follows from (p3). If (p5) does not hold, there exists a non-endpoint node $X_r$ on the path $\pi_{\mathcal{G}}(X_1, X_2, \dots, X_q)$ such that $X_r \in \mathbf{Nd}_{\mathcal{H}}(X_q) \setminus \mathbf{Pa}_{\mathcal{H}}(X_q)$. Then the triple $(X_r, X_q, \pi_{\mathcal{G}}(X_r, \dots, X_q))$ contradicts the choice of the triple $(X_1, X_q, \pi_{\mathcal{G}}(X_1, X_2, \dots, X_q))$, since $\pi_{\mathcal{G}}(X_r, \dots, X_q)$ is also open given $\mathbf{Pa}_{\mathcal{H}}(X_q)$, contains at most $m$ colliders, and contains fewer nodes than $\pi_{\mathcal{G}}(X_1, X_2, \dots, X_q)$.

To prove (p6), let $X_s \in \mathbf{Pa}_{\mathcal{H}}(X_q)$. If $X_{s-1} \in \mathbf{Adj}_{\mathcal{G}}(X_{s+1})$, then (a1) implies $X_{s-1} \in \mathbf{Adj}_{\mathcal{H}}(X_{s+1})$. Otherwise, we will use (a2) to show $X_{s-1} \in \mathbf{Adj}_{\mathcal{H}}(X_{s+1})$. The fact that $X_{s-1}$ and $X_{s+1}$ are non-adjacent in $\mathcal{G}$ and (p4) imply $\pi_{\mathcal{G}}(X_{s-1}, X_s, X_{s+1})$ is a v-structure. Thus it remains to show that $\pi_{\mathcal{H}}(X_{s-1}, X_s, X_{s+1})$ is a non-collider path in order to apply (a2). Since $\pi_{\mathcal{G}}(X_{s-1}, X_s, X_{s+1})$ is a v-structure, neither $X_{s-1}$ nor $X_{s+1}$ can be a collider on $\pi_{\mathcal{G}}(X_1, X_2, \dots, X_q)$. Therefore, (p4) implies $X_{s-1}, X_{s+1} \notin \mathbf{Pa}_{\mathcal{H}}(X_q)$. Therefore, by (p5), $\{X_{s-1}, X_{s+1}\} \subseteq \mathbf{De}_{\mathcal{H}}(X_q) \subseteq \mathbf{De}_{\mathcal{H}}(X_s)$, where the last set-inclusion follows from $X_s \in \mathbf{Pa}_{\mathcal{H}}(X_q)$. Thus, by acyclicity, $\pi_{\mathcal{H}}(X_{s-1}, X_s, X_{s+1})$ is a non-collider path and hence, (p6) follows from (a2).

Using (p1) - (p6) and Lemma 9.4, we complete the proof by showing that there exists a triple of nodes $\{X_i, X_j, X_k\}$ on the path $\pi_{\mathcal{G}}(X_1, X_2, \dots, X_q)$ such that $X_i \in \mathbf{Nd}_{\mathcal{H}}(X_k) \setminus \mathbf{Pa}_{\mathcal{H}}(X_k)$, $\pi_{\mathcal{H}}(X_i, X_j, X_k)$ is a v-structure and $X_i \not\perp_{\mathcal{G}} X_k \mid \mathbf{Pa}_{\mathcal{H}}(X_k)$.

Note that (p1) and (p6) together imply that there is a path in $\mathcal{H}$ between $X_1$ and $X_q$ through $\{X_2, \dots, X_{q-1}\} \setminus \mathbf{Pa}_{\mathcal{H}}(X_q)$. Since $X_1 \perp_{\mathcal{H}} X_q \mid \mathbf{Pa}_{\mathcal{H}}(X_q)$ (see (p2)), any path in $\mathcal{H}$

between $X_1$ and $X_q$ through any subset of $\{X_2, \ldots, X_{q-1}\} \backslash \mathbf{Pa}_{\mathcal{H}}(X_q)$ must contain a collider. Therefore, by Lemma 9.4, there exists a triple $\{X_i, X_j, X_k\} \subseteq \{X_1, \ldots, X_q\} \backslash \mathbf{Pa}_{\mathcal{H}}(X_q)$ with $1 \leq i < k \leq q$, such that $\pi_{\mathcal{H}}(X_i, X_j, X_k)$ is a v-structure and

$$\text{for all } r \in \{i+1, \ldots, k-1\},\ X_r \notin \mathbf{Pa}_{\mathcal{H}}(X_q) \text{ implies } X_r \in \mathbf{De}_{\mathcal{H}}(X_i) \cap \mathbf{De}_{\mathcal{H}}(X_k). \quad (1)$$

Below, we separately consider the following two cases: (i) $X_i \in \mathbf{Nd}_{\mathcal{H}}(X_k)$ and (ii) $X_i \in \mathbf{De}_{\mathcal{H}}(X_k)$. We will complete the proof by showing that the result holds with the ordered triples $(X_i, X_j, X_k)$ and $(X_k, X_j, X_i)$ for Case (i) and Case (ii) respectively.

**Case (i):** Suppose $X_i \in \mathbf{Nd}_{\mathcal{H}}(X_k)$. Since $\pi_{\mathcal{H}}(X_i, X_j, X_k)$ is a v-structure, $X_i$ and $X_k$ are non-adjacent in $\mathcal{H}$. Hence, $X_i \in \mathbf{Nd}_{\mathcal{H}}(X_k) \setminus \mathbf{Pa}_{\mathcal{H}}(X_k)$. Thus it remains to show that $X_i \not\perp_{\mathcal{G}} X_k \mid \mathbf{Pa}_{\mathcal{H}}(X_k)$. In fact, we show below that the subpath $\pi_{\mathcal{G}}(X_i, \ldots, X_k)$ of $\pi_{\mathcal{G}}(X_1, X_2, \ldots, X_q)$ is open given $\mathbf{Pa}_{\mathcal{H}}(X_k)$, i.e. the following conditions hold:

**(c1)** if $X_r$ is a non-collider on the path $\pi_{\mathcal{G}}(X_i, \ldots, X_k)$, then $X_r \notin \mathbf{Pa}_{\mathcal{H}}(X_k)$, and

**(c2)** if $X_s$ is a collider on the path $\pi_{\mathcal{G}}(X_i, \ldots, X_k)$, then $\mathbf{De}_{\mathcal{G}}(X_s) \cap \mathbf{Pa}_{\mathcal{H}}(X_k) \neq \emptyset$.

By (p4), if $X_r$ is a non-collider on the path $\pi_{\mathcal{G}}(X_i, \ldots, X_k)$ (and hence on the path $\pi_{\mathcal{G}}(X_1, X_2, \ldots, X_q)$), $X_r \notin \mathbf{Pa}_{\mathcal{H}}(X_q)$. Therefore, by (1), $X_r \in \mathbf{De}_{\mathcal{H}}(X_k)$. This implies $X_r \notin \mathbf{Pa}_{\mathcal{H}}(X_k)$ as $\mathcal{H}$ is acyclic. This shows (c1).

Suppose (c2) does not hold. Let $s^*$ be the largest integer such that

$$X_{s^*} \text{ is a collider on } \pi_{\mathcal{G}}(X_i, \ldots, X_k) \text{ and } \mathbf{De}_{\mathcal{G}}(X_{s^*}) \cap \mathbf{Pa}_{\mathcal{H}}(X_k) = \emptyset. \quad (2)$$

Since $X_{s^*}$ is also a collider on $\pi_{\mathcal{G}}(X_1, X_2, \ldots, X_q)$, (p3) implies $\mathbf{De}_{\mathcal{G}}(X_{s^*}) \cap \mathbf{Pa}_{\mathcal{H}}(X_q) \neq \emptyset$. Therefore, we can choose $X_{s'} \in \mathbf{De}_{\mathcal{G}}(X_{s^*}) \cap \mathbf{Pa}_{\mathcal{H}}(X_q)$ and a directed path $\pi_{\mathcal{G}}(X_{s^*}, \ldots, X_{s'})$ from $X_{s^*}$ to $X_{s'}$ in $\mathcal{G}$. Note that $X_{s'} \neq X_k$, since $X_k \notin \mathbf{Pa}_{\mathcal{H}}(X_q)$. We concatenate the paths $\pi_{\mathcal{G}}(X_k, X_{k-1}, \ldots, X_{s^*})$ and $\pi_{\mathcal{G}}(X_{s^*}, \ldots, X_{s'})$ to obtain a path $\pi^*_{\mathcal{G}}(X_k, \ldots, X_{s'})$, by avoiding possible loops, as follows: if $X_s$ is the first node in $\pi_{\mathcal{G}}(X_k, X_{k-1}, \ldots, X_{s^*})$ that intersects $\pi_{\mathcal{G}}(X_{s^*}, \ldots, X_{s'})$, then we consider the path $\pi_{\mathcal{G}}(X_k, X_{k-1}, \ldots, X_s, \ldots, X_{s'})$.

We show below that $X_{s'} \in \mathbf{Nd}_{\mathcal{H}}(X_k) \setminus \mathbf{Pa}_{\mathcal{H}}(X_k)$, and that the concatenated path $\pi^*_{\mathcal{G}}(X_k, \ldots, X_{s'})$ contains at most $m-1$ colliders and is open given $\mathbf{Pa}_{\mathcal{H}}(X_k)$. This contradicts the choice of the triple $(X_1, X_q, \pi_{\mathcal{G}}(X_1, X_2, \ldots, X_q))$. Thus (c2) must hold.

First, we prove $X_{s'} \in \mathbf{Nd}_{\mathcal{H}}(X_k) \setminus \mathbf{Pa}_{\mathcal{H}}(X_k)$. Note that $X_{s'} \notin \mathbf{Pa}_{\mathcal{H}}(X_k)$ follows from (2), since $X_{s'}$ is a descendant of $X_{s^*}$. To prove $X_{s'} \in \mathbf{Nd}_{\mathcal{H}}(X_k)$, we recall that $X_k \in \{X_2, \ldots, X_q\} \setminus \mathbf{Pa}_{\mathcal{H}}(X_q)$. Thus (p5) implies $X_k \in \mathbf{De}_{\mathcal{H}}(X_q)$, since $X_k \in \mathbf{De}_{\mathcal{H}}(X_q)$ holds trivially for $k = q$. Moreover, since $X_{s'} \in \mathbf{Pa}_{\mathcal{H}}(X_q)$, we have $\mathbf{De}_{\mathcal{H}}(X_q) \subseteq \mathbf{De}_{\mathcal{H}}(X_{s'})$. Hence, $X_k \in \mathbf{De}_{\mathcal{H}}(X_{s'})$ implies $X_{s'} \in \mathbf{Nd}_{\mathcal{H}}(X_k)$ (as $X_{s'} \neq X_k$).

Next, note that the concatenated path $\pi^*_{\mathcal{G}}(X_k, \ldots, X_{s'})$ contains at most $m-1$ colliders follows from the fact that $\pi_{\mathcal{G}}(X_k, X_{k-1}, \ldots, X_{s^*})$ contains at most $m-1$ colliders and the directed path $\pi_{\mathcal{G}}(X_{s^*}, \ldots, X_{s'})$ contains no collider.

Finally, using (c1) and (2), we show that the concatenated path $\pi^*_{\mathcal{G}}(X_k, \ldots, X_{s'})$ is open given $\mathbf{Pa}_{\mathcal{H}}(X_k)$, i.e. the following conditions hold:

**(c1*)** if $X_r$ is a non-collider on the path $\pi^*_{\mathcal{G}}(X_k,\ldots,X_{s'})$, then $X_r \notin \mathbf{Pa}_{\mathcal{H}}(X_k)$, and

**(c2*)** if $X_s$ is a collider on the path $\pi^*_{\mathcal{G}}(X_k,\ldots,X_{s'})$, then $\mathbf{De}_{\mathcal{G}}(X_s) \cap \mathbf{Pa}_{\mathcal{H}}(X_k) \neq \emptyset$.

If $X_r$ is a non-collider on the concatenated path $\pi^*_{\mathcal{G}}(X_k,\ldots,X_{s'})$, then $X_r$ is either a non-collider on $\pi_{\mathcal{G}}(X_k,X_{k-1},\ldots,X_{s^*})$ or $X_r$ intersects the directed path $\pi_{\mathcal{G}}(X_{s^*},\ldots,X_{s'})$. If $X_r$ is a non-collider on $\pi_{\mathcal{G}}(X_k,X_{k-1},\ldots,X_{s^*})$, then (c1) implies $X_r \notin \mathbf{Pa}_{\mathcal{H}}(X_k)$. If $X_r$ intersects the directed path $\pi_{\mathcal{G}}(X_{s^*},\ldots,X_{s'})$, then $X_r \in \mathbf{De}_{\mathcal{G}}(X_{s^*})$. Hence, $X_r \notin \mathbf{Pa}_{\mathcal{H}}(X_k)$, by (2).

If $X_s$ is collider on the concatenated path $\pi_{\mathcal{G}}(X_k,\ldots,X_{s'})$, then $X_s$ must be a collider on $\pi_{\mathcal{G}}(X_k,X_{k-1},\ldots,X_{s^*})$ (as $\pi_{\mathcal{G}}(X_{s^*},\ldots,X_{s'})$ is a directed path). This implies $\mathbf{De}_{\mathcal{G}}(X_s) \cap \mathbf{Pa}_{\mathcal{H}}(X_k) \neq \emptyset$, since otherwise this would contradict the fact that $s^*$ is the largest integer for which (2) holds.

**Case (ii):** Suppose $X_i \in \mathbf{De}_{\mathcal{H}}(X_k)$. This implies $X_k \in \mathbf{Nd}_{\mathcal{H}}(X_i)$ as $i \neq k$. For $X_i \in \{X_2,\ldots,X_q\} \setminus \mathbf{Pa}_{\mathcal{H}}(X_q)$, we can repeat the arguments given in Case (i) while switching the roles of $X_i$ and $X_k$. Thus we complete the proof by showing that the sub-case $X_i = X_1$ and $X_i \in \mathbf{De}_{\mathcal{H}}(X_k)$ is impossible. To this end, recall that $X_1 \in \mathbf{Nd}_{\mathcal{H}}(X_q)$. Further, by (p5), $X_k \in \mathbf{De}_{\mathcal{H}}(X_q)$. Therefore, we have $X_1 \in \mathbf{Nd}_{\mathcal{H}}(X_k)$. □

## 9.2 Proof of Corollary 4.1 of the main text

The fact that $\mathcal{H}$ is not an independence map of $\mathcal{G}_0$ implies that at least one of the three conditions of Theorem 4.1 of the main text hold. If the first condition holds, then there exists a pair of nodes $\{X_i,X_k\}$ that are adjacent in $\mathcal{G}_0$ and non-adjacent in $\mathcal{H}$. Additionally, without loss of generality, we assume that $X_i \in \mathbf{Nd}_{\mathcal{H}}(X_k)$. Since $X_i$ and $X_k$ are adjacent in $\mathcal{G}_0$, $X_i$ and $X_k$ are not d-separated by any subset of $\mathbf{X} \setminus \{X_i,X_k\}$. Therefore, $X_i \not\perp X_k \mid \mathbf{Pa}_{\mathcal{H}}(X_k)$. The admissibility of the edge $X_i \to X_k$ with respect to $\mathcal{I}_0$ and with respect to skeleton($\mathcal{C}_0$) follows from the fact that $X_i$ and $X_k$ are adjacent in $\mathcal{G}_0$, since skeleton($\mathcal{G}_0$) = skeleton($\mathcal{C}_0$) $\subseteq \mathcal{I}_0$. Therefore, the pair of nodes $\{X_i,X_k\}$ satisfies the conditions of Corollary 4.1 of the main text.

If a triple of nodes $\{X_i,X_j,X_k\}$ satisfies the second condition of Theorem 4.1 of the main text, we show that the pair $\{X_i,X_k\}$ satisfies the conditions of Corollary 4.1 of the main text, where without loss of generality, we assume that $X_i \in \mathbf{Nd}_{\mathcal{H}}(X_k)$. First, we prove $X_i \not\perp_{\mathcal{G}_0} X_k \mid \mathbf{Pa}_{\mathcal{H}}(X_k)$ by showing that the path $\pi_{\mathcal{G}_0}(X_i,X_j,X_k)$ is open given $\mathbf{Pa}_{\mathcal{H}}(X_k)$. Note that $\pi_{\mathcal{H}}(X_i,X_j,X_k)$ is a non-collider path and $X_i \in \mathbf{Nd}_{\mathcal{H}}(X_k)$ imply $\pi_{\mathcal{H}}(X_i,X_j,X_k)$ must be either $X_i \leftarrow X_j \to X_k$ or $X_i \to X_j \to X_k$. Hence, $X_j \in \mathbf{Pa}_{\mathcal{H}}(X_k)$. This implies that $\pi_{\mathcal{G}_0}(X_i,X_j,X_k)$ is open given $\mathbf{Pa}_{\mathcal{H}}(X_k)$, since $X_j$ is a collider on the path $\pi_{\mathcal{G}_0}(X_i,X_j,X_k)$. Next, we show that $X_i \to X_k$ is admissible for CPDAG($\mathcal{H}$) with respect to $\mathcal{I}_0$ and with respect to skeleton($\mathcal{C}_0$). Since $\pi_{\mathcal{G}_0}(X_i,X_j,X_k)$ is a v-structure, $X_i$ and $X_k$ are adjacent in $\mathcal{I}_0$, and hence, $X_i \to X_k$ is admissible for CPDAG($\mathcal{H}$) with respect to $\mathcal{I}_0$. $X_i \to X_k$ is admissible for CPDAG($\mathcal{H}$) with respect to skeleton($\mathcal{C}_0$) follows from the fact that $(X_i,X_j,X_k)$ is an unshielded triple in $\mathcal{H}$.

If a triple $\{X_i, X_j, X_k\}$ satisfies the third condition of Theorem 4.1 of the main text, then it is easy to see that the pair $\{X_i, X_k\}$ satisfies the conditions of Corollary 4.1 of the main text. $\square$

## 9.3 Proof of Theorem 4.2 of the main text

We show that $\lim_{n\to\infty} \mathbb{P}(\mathbb{CI}(\hat{\mathcal{C}}_n^f) \subseteq \mathbb{CI}(\mathcal{C}_0)) = 1$, where $\hat{\mathcal{C}}_n^f$ denotes the output of the forward phase of ARGES-CIG. Then $\lim_{n\to\infty} \mathbb{P}(\hat{C}_n = \mathcal{C}_0) = 1$ follows from the arguments given in Lemma 10 of Chickering [2002], as the backward phase of ARGES-CIG and GES are identical.

Let $A_n = \{\mathcal{I}_0 \subseteq \hat{\mathcal{I}}_n\}$. Thus $\lim_{n\to\infty} \mathbb{P}(A_n) = 1$ and it is sufficient to prove $\lim_{n\to\infty} \mathbb{P}(\mathbb{CI}(\hat{\mathcal{C}}_n^f) \nsubseteq \mathbb{CI}(\mathcal{C}_0), A_n) = 0$. To this end, we write

$$\mathbb{P}(\mathbb{CI}(\hat{\mathcal{C}}_n^f) \nsubseteq \mathbb{CI}(\mathcal{C}_0), A_n) = \sum_{\mathcal{C}} \mathbb{P}(\hat{\mathcal{C}}_n^f = \mathcal{C}, A_n),$$

where the sum is over all CPDAGs $\mathcal{C}$ that are not independence maps of $\mathcal{C}_0$. It is sufficient to show that for any such CPDAG $\mathcal{C}$, $\lim_{n\to\infty} \mathbb{P}(\hat{\mathcal{C}}_n^f = \mathcal{C}, A_n) = 0$, since the total number of CPDAGs that are not independence maps of $\mathcal{C}_0$ does not depend on $n$.

We fix a CPDAG $\mathcal{C}$ that is not an independence map of $\mathcal{C}_0$. Let $\mathcal{H}$ be any DAG in the Markov equivalence class of $\mathcal{C}$. Therefore, $\mathcal{H}$ is not an independence map of $\mathcal{G}_0$. Thus, by Corollary 4.1 of the main text, there exists a pair of non-adjacent nodes $\{X_i, X_k\}$ in $\mathcal{H}$ such that $X_i \in \mathbf{Nd}_{\mathcal{H}}(X_k)$, $X_i \not\perp_{\mathcal{G}_0} X_k \mid \mathbf{Pa}_{\mathcal{H}}(X_k)$ and $X_i \to X_k$ is an admissible edge for $\mathcal{C}$ with respect to $\mathcal{I}_0$. We construct the DAG $\mathcal{H}'$ from $\mathcal{H}$ by adding the edge $X_i \to X_k$. Since $X_i \not\perp_{\mathcal{G}_0} X_k \mid \mathbf{Pa}_{\mathcal{H}}(X_k)$, the local consistency property of the scoring criterion (see Definition 2.4) implies

$$\lim_{n\to\infty} \mathbb{P}(\mathcal{S}(\mathcal{H}', \mathcal{D}_n) < \mathcal{S}(\mathcal{H}, \mathcal{D}_n)) = 1.$$

We complete the proof by showing $\{\hat{\mathcal{C}}_n^f = \mathcal{C}\} \cap A_n \subseteq \{\mathcal{S}(\mathcal{H}', \mathcal{D}_n) \geq \mathcal{S}(\mathcal{H}, \mathcal{D}_n)\}$.

On the set $A_n$, the edge $X_i \to X_k$ is admissible for $\mathcal{C}$ with respect to $\hat{\mathcal{I}}_n$. This implies that the move from $\mathcal{C}$ to CPDAG$(\mathcal{H}')$ is admissible on the set $A_n$. If $\mathcal{C}$ is the output of the forward phase of ARGES-CIG, no admissible move from $\mathcal{C}$ can improve the score. Therefore, $\{\hat{\mathcal{C}}_n^f = \mathcal{C}\} \cap A_n \subseteq \{\mathcal{S}(\mathcal{H}', \mathcal{D}_n) \geq \mathcal{S}(\mathcal{H}, \mathcal{D}_n)\}$. $\square$

## 9.4 Proof of Theorem 4.3 of the main text

The proof of Theorem 4.3 of the main text follows analogously to the proof of Theorem 4.2 of the main text (see Section 9.3 above). $\square$

## 9.5 Proof of Lemma 5.1 of the main text

Since $\mathbf{Pa}_{\mathcal{H}'}(X_r) = \mathbf{Pa}_{\mathcal{H}}(X_r)$ for all $r \neq k$, and $|E_{\mathcal{H}'}| = |E_{\mathcal{H}}| + 1$,

$$\begin{aligned} \mathcal{S}_\lambda(\mathcal{H}', \mathcal{D}_n) - \mathcal{S}_\lambda(\mathcal{H}, \mathcal{D}_n) =& \frac{1}{n} \log \left( L(\hat{\boldsymbol{\theta}}_k(\mathcal{H}), \mathcal{D}_n(X_k) | \mathcal{D}_n(\mathbf{Pa}_{\mathcal{H}}(X_k))) \right) \\ & - \frac{1}{n} \log \left( L(\hat{\boldsymbol{\theta}}_k(\mathcal{H}'), \mathcal{D}_n(X_k) | \mathcal{D}_n(\mathbf{Pa}_{\mathcal{H}'}(X_k))) \right) + \lambda. \end{aligned} \quad (3)$$

The fact that the distribution of $\mathbf{X}$ is multivariate Gaussian implies that the conditional distribution of $X_k$ given $\mathbf{Pa}_{\mathcal{H}}(X_k)$ is $\mathcal{N}(\mu_k^* + \boldsymbol{\beta}_k^*(\mathcal{H})^T \mathbf{Pa}_{\mathcal{H}}(X_k), \sigma_k^*(\mathcal{H})^2)$, where $\mathrm{E}[X_k \mid \mathbf{Pa}_{\mathcal{H}}(X_k)] = \mu_k^* + \boldsymbol{\beta}_k^*(\mathcal{H})^T \mathbf{Pa}_{\mathcal{H}}(X_k)$ and $\mathrm{Var}[X_k \mid \mathbf{Pa}_{\mathcal{H}}(X_k)] = \sigma_k^*(\mathcal{H})^2$.

Let $\mathbf{x}_s = (x_{1,s}, \ldots, x_{p,s})^T$ be the $s$-th sample in $\mathcal{D}_n$ and let $\mathbf{Pa}_{\mathcal{H}}(x_{k,s})$ denote the sub-vector of $\mathbf{x}_s$ that corresponds to $\mathbf{Pa}_{\mathcal{H}}(X_k)$. Therefore,

$$\begin{aligned} & \frac{1}{n} \log \left( L((\mu_k, \boldsymbol{\beta}_k(\mathcal{H})^T, \sigma_k(\mathcal{H})), \mathcal{D}_n(X_k) | \mathcal{D}_n(\mathbf{Pa}_{\mathcal{H}}(X_k))) \right) \\ =& -\frac{1}{2} \log(2\pi\sigma_k(\mathcal{H})^2) - \frac{1}{2n\sigma_k(\mathcal{H})^2} \sum_{s=1}^{n} \left( x_{k,s} - \mu_k(\mathcal{H}) - \boldsymbol{\beta}_k(\mathcal{H})^T \mathbf{Pa}_{\mathcal{H}}(x_{k,s}) \right)^2. \end{aligned} \quad (4)$$

Thus the MLE $(\hat{\mu}_k, \hat{\boldsymbol{\beta}}_k(\mathcal{H})^T)$ of $(\mu_i, \boldsymbol{\beta}_k(\mathcal{H})^T)$ is the vector of sample regression coefficients in the regression (with intercept) of $X_k$ on $\mathbf{Pa}_{\mathcal{H}}(X_k)$, and the MLE of $\sigma_k(\mathcal{H})^2$ equals

$$\hat{\sigma}_k(\mathcal{H})^2 = \frac{1}{n} \sum_{s=1}^{n} \left( x_{k,s} - \hat{\mu}_k - \hat{\boldsymbol{\beta}}_k(\mathcal{H})^T \mathbf{Pa}_{\mathcal{H}}(x_{k,s}) \right)^2.$$

Hence, from (4), we have,

$$\frac{1}{n} \log \left( L((\hat{\mu}_k, \hat{\boldsymbol{\beta}}_k(\mathcal{H})^T, \hat{\sigma}_k(\mathcal{H})), \mathcal{D}_n(X_k) | \mathcal{D}_n(\mathbf{Pa}_{\mathcal{H}}(X_k))) \right) = -\frac{1}{2} \log(2\pi\hat{\sigma}_k(\mathcal{H})^2) - \frac{1}{2}. \quad (5)$$

By combining (3) and (5), we obtain,

$$\mathcal{S}_\lambda(\mathcal{H}', \mathcal{D}_n) - \mathcal{S}_\lambda(\mathcal{H}, \mathcal{D}_n) = \frac{1}{2} \log \left( \frac{\hat{\sigma}_k(\mathcal{H}')^2)}{\hat{\sigma}_k(\mathcal{H})^2)} \right) + \lambda.$$

Since $\hat{\sigma}_k(\mathcal{H})^2$ is the variance of the residuals in the regression of $X_k$ on $\mathbf{Pa}_{\mathcal{H}}(X_k)$, and $\hat{\sigma}_k(\mathcal{H}')^2$ is the variance of the residuals in the regression of $X_k$ on $\mathbf{Pa}_{\mathcal{H}}(X_k) \cup \{X_i\}$, $\hat{\sigma}_k(\mathcal{H}')^2 = \left( 1 - \hat{\rho}^2_{ik|\mathbf{Pa}_{\mathcal{H}}(k)} \right) \hat{\sigma}_k(\mathcal{H})^2$ [Yule, 1907]. Therefore,

$$\mathcal{S}_\lambda(\mathcal{H}', \mathcal{D}_n) - \mathcal{S}_\lambda(\mathcal{H}, \mathcal{D}_n) = \frac{1}{2} \log \left( 1 - \hat{\rho}^2_{ik|\mathbf{Pa}_{\mathcal{H}}(k)} \right) + \lambda.$$

□

## 9.6 Proof of Theorem 5.1 of the main text

The following lemma will be used to prove Theorem 5.1 of the main text.

**Lemma 9.5.** *Let $\mathcal{H} = (\mathbf{X}, E)$ be a DAG such that $X_i \to X_k \in E$. Let $\mathcal{H}' = (\mathbf{X}, E \setminus \{X_i \to X_k\})$. If $\mathcal{H}$ is an independence map of $\mathcal{G}_0$ but $\mathcal{H}'$ is not, then $X_i \not\perp\!\!\!\perp X_k \mid \mathbf{Pa}_{\mathcal{H}'}(X_i)$.*

*Proof.* Since $\mathcal{G}_0$ is a perfect map of the distribution of $\mathbf{X}$, a DAG $\mathcal{H}$ is an independence map of $\mathcal{G}_0$ if and only if all conditional independence constraints encoded by $\mathcal{H}$ hold in the distribution of $\mathbf{X}$. Therefore, $\mathcal{H}$ is an independence map of $\mathcal{G}_0$ if and only if the joint density of $\mathbf{X}$ factorizes according to $\mathcal{H}$ (see Theorem 3.27 of Lauritzen [1996]).

Hence, the joint density $f(x_1, \dots, x_p)$ satisfies

$$f(x_1, \dots, x_p) = \prod_{r=1}^{p} f_r(x_r \mid \mathbf{Pa}_{\mathcal{H}}(X_r) = \mathbf{Pa}_{\mathcal{H}}(x_r)),$$

where $\mathbf{Pa}_{\mathcal{H}}(x_r)$ is the sub-vector of $(x_1, \dots, x_p)$ that corresponds to $\mathbf{Pa}_{\mathcal{H}}(X_r)$.

Suppose $X_i \perp\!\!\!\perp X_k \mid \mathbf{Pa}_{\mathcal{H}'}(X_k)$. This implies that the conditional density of $X_k$ given $\mathbf{Pa}_{\mathcal{H}}(X_k)$ is identical to the conditional density of $X_k$ given $\mathbf{Pa}_{\mathcal{H}'}(X_k) = \mathbf{Pa}_{\mathcal{H}}(X_k) \setminus \{X_i\}$. Moreover, for all $r \neq k$,

$$f_r(x_r \mid \mathbf{Pa}_{\mathcal{H}}(X_r) = \mathbf{Pa}_{\mathcal{H}}(x_r)) = f_r(x_r \mid \mathbf{Pa}_{\mathcal{H}'}(X_r) = \mathbf{Pa}_{\mathcal{H}'}(x_r)),$$

since $\mathbf{Pa}_{\mathcal{H}}(X_r) = \mathbf{Pa}_{\mathcal{H}'}(X_r)$.

Thus the joint density also factorizes according to $\mathcal{H}'$. This contradicts the fact that $\mathcal{H}'$ is not an independence map of $\mathcal{G}_0$. □

**Proof of Theorem 5.1 of the main text.** Fix a $\lambda$ satisfying $\lambda < -\frac{1}{2}\log(1 - \rho^2_{ij|S})$ for all $i, j \in \{1, \dots, p\}$ and $S \subseteq \{1, \dots, p\} \setminus \{i, j\}$ such that $|S| \leq m$ and $\rho_{ij|S} \neq 0$. Let $\delta \in [0, 1]$ and fix a $\delta$-optimal oracle version of ARGES with scoring criterion $\mathcal{S}^*_\lambda$, and let $\mathcal{C}^f$ and $\mathcal{C}^*$ denote the output of the forward phase and the final output respectively. Thus, we have $\mathbf{Adj}_{\mathcal{C}^f}(X_k) \leq m$, for all $k \in \{1, \dots, p\}$.

First, we show that $\mathcal{C}^f$ is an independence map of $\mathcal{C}_0$ (cf. Lemma 9 of Chickering, 2002). Let $\mathcal{H} = (\mathbf{X}, E)$ be any DAG in the Markov equivalence class of $\mathcal{C}^f$. If $\mathcal{H}$ is not an independence map of $\mathcal{G}_0$, then by Corollary 4.1 of the main text, there exists a pair of nodes $(X_i, X_k)$ such that $X_i \in \mathbf{Nd}_{\mathcal{H}}(X_k) \setminus \mathbf{Pa}_{\mathcal{H}}(X_k)$, $X_i \not\perp_{\mathcal{G}_0} X_k \mid \mathbf{Pa}_{\mathcal{H}}(X_k)$ and the edge $X_i \to X_k$ is admissible for $\mathcal{C}^f$ with respect to $\mathcal{I}_0$ (for ARGES-CIG), with respect to skeleton $\mathcal{C}_0$ (for ARGES-skeleton) or with respect to the complete undirected graph (for GES). Let $\mathcal{H}' = (\mathbf{X}, E \cup \{X_i \to X_k\})$ and note that $X_i \not\perp_{\mathcal{G}_0} X_k \mid \mathbf{Pa}_{\mathcal{H}}(X_k)$ implies $\rho_{ik|\mathbf{Pa}_{\mathcal{H}}(k)} \neq 0$. Therefore, by Lemma 5.2 of the main text, $\mathcal{S}^*_\lambda(\mathcal{H}', F) - \mathcal{S}^*_\lambda(\mathcal{H}, F) < 0$, since $\lambda < -\frac{1}{2}\log(1 - \rho^2_{ik|\mathbf{Pa}_{\mathcal{H}}(k)})$ as $|\mathbf{Pa}_{\mathcal{H}}(X_k)| \leq m$. This contradicts the fact that $\mathcal{C}^f$ is the output of the forward phase.

Next, we show that $\mathcal{C}^*$ is an independence map of $\mathcal{C}_0$ given that $\mathcal{C}^f$ is an independence map of $\mathcal{C}_0$ (cf. Lemma 10 of Chickering, 2002). Suppose not, then there must be a transition

from a CPDAG $\mathcal{C}$ to $\mathcal{C}'$ in the backward phase of the oracle version such that $\mathcal{C}$ is an independence map of $\mathcal{C}_0$ but $\mathcal{C}'$ is not. Let $\mathcal{H}$ and $\mathcal{H}'$ be two DAGs in the Markov equivalence classes of $\mathcal{C}$ and $\mathcal{C}'$ respectively, such that $\mathcal{H}'$ can be obtained from $\mathcal{H}$ by deleting exactly one edge $X_i \to X_k$ (see line 4 of Algorithm 3.2). Then by Lemma 9.5, $X_i \not\perp\!\!\!\perp X_k \mid \mathbf{Pa}_{\mathcal{H}'}(X_k)$. Hence $\rho_{ik|\mathbf{Pa}_{\mathcal{H}'}(k)} \neq 0$ and by Lemma 5.2 of the main text, $\mathcal{S}^*_\lambda(\mathcal{H}', F) > \mathcal{S}^*_\lambda(\mathcal{H}, F)$, since $\lambda < -\frac{1}{2}\log(1-\rho^2_{ik|\mathbf{Pa}_{\mathcal{H}'}(k)})$ as $|\mathbf{Pa}_{\mathcal{H}'}(X_k)| \leq m$. This is a contradiction.

Finally, we show that $\mathcal{C}^* = \mathcal{C}_0$ given that $\mathcal{C}^*$ is an independence map of $\mathcal{C}_0$ (cf. Lemma 10 of Chickering, 2002). Suppose $\mathcal{C}^* \neq \mathcal{C}_0$. Let $\mathcal{H}^*$ be a DAG in the Markov equivalence class of $\mathcal{C}^*$. Thus $\mathcal{H}^*$ is an independence map of $\mathcal{G}_0$. Therefore, by Theorem 4 of Chickering [2002], there exists a sequence of covered edge reversals and edge additions that transforms $\mathcal{G}_0$ to $\mathcal{H}^*$ such that each DAG obtained in the sequence is an independence map of $\mathcal{G}_0$, where an edge $X_r \to X_s$ is said to be covered in a DAG $\mathcal{H}$ if $\mathbf{Pa}_{\mathcal{H}}(X_s) = \mathbf{Pa}_{\mathcal{H}}(X_r) \cup \{X_r\}$. Moreover, there must be at least one edge addition in the sequence, since otherwise $\mathcal{H}^*$ and $\mathcal{G}_0$ must be in the same equivalence class (by Lemma 1 of Chickering, 1995). Consider the DAG $\mathcal{H}$ that precedes the last edge addition $X_i \to X_k$ in the sequence. We complete the proof by showing that the score can be improved by moving from $\mathcal{C}^*$ to the Markov equivalence class of $\mathcal{H}$ by a single edge deletion. This contradicts the fact that $\mathcal{C}^*$ is the final output.

Let $\mathcal{H}'$ be the DAG that is obtained from $\mathcal{H}$ by adding the edge $X_i \to X_k$ to $\mathcal{H}$. Since $\mathcal{H}$ is an independence map of $\mathcal{G}_0$ and $X_i \perp_{\mathcal{H}} X_k \mid \mathbf{Pa}_{\mathcal{H}}(X_k)$, we have $X_i \perp_{\mathcal{G}_0} X_k \mid \mathbf{Pa}_{\mathcal{H}}(X_k)$. Hence $\rho_{ik|\mathbf{Pa}_{\mathcal{H}}(k)} = 0$, since $\mathcal{G}_0$ is a perfect map. Therefore, by Lemma 5.2 of the main text, $\mathcal{S}^*_\lambda(\mathcal{H}', F) - \mathcal{S}^*_\lambda(\mathcal{H}, F) = \lambda > 0$. Since $\mathcal{H}^*$ can be obtained from $\mathcal{H}'$ by covered edge reversals, by Lemma 1 of Chickering [1995], they belong to the same Markov equivalence class. Therefore, $\mathcal{S}^*_\lambda(\mathcal{H}^*, F) = \mathcal{S}^*_\lambda(\mathcal{H}', F)$ as $\mathcal{S}^*_\lambda$ is score equivalent. Hence $\mathcal{S}^*_\lambda(\mathcal{H}^*, F) = \mathcal{S}^*_\lambda(\mathcal{H}', F) > \mathcal{S}^*_\lambda(\mathcal{H}, F)$. This implies that the score can be improved by moving from $\mathcal{C}^*$ to CPDAG($\mathcal{H}$). □

## 9.7 Proof of Theorem 5.2 of the main text

The following result was applied to prove high-dimensional consistency of the PC algorithm [Kalisch and Bühlmann, 2007]. We will also use it to prove Theorems 5.2 of the main text.

**Proposition 9.1.** *(Corollary 1 of Kalisch and Bühlmann, 2007) Assume the first part of (A1) and the upper bound in (A6). Let $\hat{\rho}_{nij|S}$ denote the sample partial correlation between $X_{ni}$ and $X_{nj}$ given $\{X_{nr} : r \in S\}$ based on $\mathcal{D}_n$, and let $\mathbf{S}^{m_n}_{i,j} = \{S \subseteq \{1, \ldots, p_n\} \setminus \{i,j\} : |S| \leq m_n\}$. Then for any $\delta > 0$,*

$$\sup_{i,j,S\in\mathbf{S}^{m_n}_{i,j}} \mathbb{P}\left(\left|\hat{\rho}_{nij|S} - \rho_{nij|S}\right| > \delta\right) \leq C_1(n-2-m_n)\exp\left((n-4-m_n)\log\left(\frac{4-\delta^2}{4+\delta^2}\right)\right),$$

*for some constant $0 < C_1 < \infty$ depending on $M$ from (A6) only.*

**Corollary 9.1.** *Assume the conditions of Proposition 9.1. Let $S_{i,j}^{m_n}$ be as in Proposition 9.1 and let $h(\rho) = (-0.5\log(1-\rho^2))^{1/2}$. Then for any $\delta > 0$,*

$$\sup_{i,j,S\in\mathbf{S}_{i,j}^{m_n}} \mathbb{P}\left(\left|h(\hat{\rho}_{nij|S}) - h(\rho_{nij|S})\right| > \delta\right)$$
$$\leq \mathcal{O}(n-m_n)\exp\left((n-4-m_n)\log\left(\frac{4-(\delta/L)^2}{4+(\delta/L)^2}\right) + \exp(-C_2(n-m_n))\right), \quad (6)$$

*for some constants $0 < C_2 < \infty$ and $L = 1/(1-(1+M)^2/4)$.*

*Proof.* We note that the result can be proved similarly as Lemma 3 of Kalisch and Bühlmann [2007]. Thus, we discuss the main idea and point out why our result holds with the same constants as in Lemma 3 of Kalisch and Bühlmann [2007].

Kalisch and Bühlmann [2007] showed that the upper bound in (6) holds for the function $g(\rho) = 0.5\log((1+\rho)/(1-\rho))$. The main idea of the proof was to apply the mean value theorem to obtain

$$g(\hat{\rho}_{nij|S}) - g(\rho_{nij|S}) = g'(\tilde{\rho}_{nij|S})(\hat{\rho}_{nij|S} - \rho_{nij|S}),$$

where $|\tilde{\rho}_{nij|S} - \rho_{nij|S}| < |\hat{\rho}_{nij|S} - \rho_{nij|S}|$. The rest of the proof obtains (uniform) upper bounds on $\mathbb{P}(|g'(\tilde{\rho}_{nij|S})| > L)$ and $\mathbb{P}(|\hat{\rho}_{nij|S} - \rho_{nij|S}| > \delta/L)$ separately, and finally combine the upper bounds to obtain the upper bound given in (6).

We can apply the same technique but with $h(\rho) = (-0.5\log(1-\rho^2))^{1/2}$. Moreover, note that

$$0 \leq h'(\rho) = \frac{1}{2\sqrt{-0.5\log(1-\rho^2)}}\frac{\rho}{1-\rho^2} = \frac{1}{\sqrt{2}}\frac{\rho}{\sqrt{-\log(1-\rho^2)}}g'(\rho) \leq \frac{g'(\rho)}{\sqrt{2}},$$

where the last inequality follows from the fact that $\sqrt{-\log(1-\rho^2)} \geq \rho$. for all $0 < \rho < 1$. Therefore, $\mathbb{P}(|h'(\tilde{\rho}_{nij|S})| > L) \leq \mathbb{P}(|g'(\tilde{\rho}_{nij|S})| > L)$. This shows that the upper bound given in Lemma 3 of Kalisch and Bühlmann [2007] also holds for the function $h(\rho)$ with the same constants. □

**Proof of Theorem 5.2 of the main text.** (cf. Lemma 4 of Kalisch and Bühlmann, 2007)

Let $A_n = \{\hat{\mathcal{I}}_n \neq \mathcal{I}_{n0}\}$ (for ARGES-CIG), $A_n = \{\hat{\mathcal{U}}_n \neq \text{skeleton}(\mathcal{C}_{n0})\}$ (for ARGES-skeleton) or $A_n = \emptyset$ (for GES). It suffices to show that $\lim_{n\to\infty} \mathbb{P}(\hat{\mathcal{C}}_n \neq \mathcal{C}_{n0}, A_n^{\mathrm{c}}) = 0$, since by assumption (A4), $\lim_{n\to\infty} \mathbb{P}(A_n^{\mathrm{c}}) = 1$.

We choose $\lambda_n = -\frac{1}{9}\log(1-c_n^2)$, where $c_n$ is given by (A6) and we define the set

$$E_{nij|S} := \{\left|h(\hat{\rho}_{nij|S}) - h(\rho_{nij|S})\right| > \sqrt{\lambda_n}\} \cup \{|\hat{\rho}_{nij|S} - \rho_{nij|S}| > \delta_n/2\},$$

for $i \neq j$ and $S \subseteq \{1,\ldots,p_n\} \setminus \{i,j\}$, where $\delta_n$ is given by assumption (A5), $h(\rho) = (-0.5\log(1-\rho^2))^{1/2}$ and $\hat{\rho}_{nij|S}$ denote the sample partial correlation between $X_{ni}$ and $X_{nj}$ given $\{X_{nr} : r \in S\}$. Further, we define

$$\mathbf{S}_{i,j}^{K_n q_n} := \{S \subseteq \{1,\ldots,p_n\} \setminus \{i,j\} : |S| \leq K_n q_n\}.$$

We will show below that

$$\mathbb{P}(\hat{\mathcal{C}}_n \neq \mathcal{C}_{n0}, A_n^{\mathsf{c}}) \leq \sum_{i,j,S\in\mathbf{S}_{i,j}^{K_n q_n}} \mathbb{P}(E_{nij|S}). \tag{7}$$

Finally, we will apply Corollary 9.1 to show that the right-hand side of (7) converges to zero.

We prove (7) by applying Lemma 5.1 and Theorem 5.1 of the main text. Note that by assumption (A6), for all $i \neq j$ and $S \in \mathbf{S}_{i,j}^{K_n q_n}$ such that $\rho_{nij|S} \neq 0$, we have,

$$\lambda_n = -\frac{1}{9}\log(1-c_n^2) < -\frac{1}{2}\log(1-c_n^2) \leq -\frac{1}{2}\log\left(1-\rho_{nij|S}^2\right).$$

Therefore, assumption (A5) and Theorem 5.1 assure that the outputs of all $\delta_n$-optimal oracle versions of (AR)GES are identical and equal to $\mathcal{C}_{n0}$ for all $n$.

Note that $\mathbb{P}(\hat{\mathcal{C}}_n \neq \mathcal{C}_{n0}, A_n^{\mathsf{c}})$ is bounded by the probability of the event $E$ that on the set $A_n^{\mathsf{c}}$ the sample version of (AR)GES makes at least one "wrong move" that cannot be made by a $\delta_n$-optimal oracle version of (AR)GES.

Lemma 5.1 of the main text implies that the sample version of (AR)GES cannot make any wrong move if the following conditions hold for all $i \neq j$ and $S \in \mathbf{S}_{i,j}^{K_n q_n}$:

**(C1)** if $\rho_{nij|S} = 0$, then $0.5\log(1-\hat{\rho}_{nij|S}^2) + \lambda_n \geq 0$,

**(C2)** if $\rho_{nij|S} \neq 0$, then $0.5\log(1-\hat{\rho}_{nij|S}^2) + \lambda_n < 0$,

**(C3)** if $\rho_{nij|S} \neq 0$, then $|\hat{\rho}_{nij|S} - \rho_{nij|S}| \leq \delta_n/2$.

**(C1)** ensures that (AR)GES does not add any edge in the forward phase for which the corresponding partial correlation is zero, and always deletes an edge in the backward phase for which the corresponding partial correlation is zero. **(C2)** ensures that (AR)GES chooses an optimal move in the sample version that is associated with a nonzero population partial correlation at every step in the forward phase, while **(C3)** makes sure that the optimal sample move corresponds to a move of a $\delta_n$-optimal oracle version.

Since $h(0) = 0$, **(C1)** is equivalent to the following condition: if $\rho_{nij|S} = 0$, then $|h(\hat{\rho}_{nij|S}) - h(\rho_{nij|S})| \leq \sqrt{\lambda_n}$. Since $h(\rho) = (-0.5\log(1-\rho^2))^{1/2}$ is an increasing function, by definition of $c_n$ (see assumption (A6)) and by the choice of $\lambda_n$, $h(\rho_{nij|S}) \geq h(c_n) > 2\sqrt{\lambda_n}$ for all $i \neq j$ and $S \in \mathbf{S}_{i,j}^{K_n q_n}$ such that $\rho_{nij|S} \neq 0$. Therefore, **(C2)** (which is equivalent to the condition: if $\rho_{nij|S} \neq 0$, then $h(\hat{\rho}_{nij|S}) > \sqrt{\lambda_n}$) is implied by the following condition: $\rho_{nij|S} \neq 0$, $|h(\hat{\rho}_{nij|S}) - h(\rho_{nij|S})| \leq \sqrt{\lambda_n}$. Thus

$$\bigcap_{i,j,S\in\mathbf{S}_{i,j}^{K_n q_n}} E_{nij|S}^{\mathsf{c}} \subseteq E^{\mathsf{c}} = \{\text{(AR)GES does not make a wrong move on the set } A_n^{\mathsf{c}}\}.$$

Hence, we have

$$\mathbb{P}(\hat{\mathcal{C}}_n \neq \mathcal{C}_{n0}, A_n^{\mathsf{c}}) \leq \mathbb{P}(E) \leq \mathbb{P}\Big(\bigcup_{i,j,S\in\mathbf{S}_{i,j}^{K_n q_n}} E_{nij|S}\Big) \leq \sum_{i,j,S\in\mathbf{S}_{i,j}^{K_n q_n}} \mathbb{P}(E_{nij|S}).$$

Using Proposition 9.1, Corollary 9.1, and the fact that $\log(\frac{4-\delta^2}{4+\delta^2}) \sim \delta^2/2$ as $\delta \to 0$, for sufficiently large $n$, we have

$$\sup_{i,j,S\in\mathbf{S}_{i,j}^{K_n q_n}} \mathbb{P}(E_{nij|S}) \leq \mathcal{O}(n - K_n q_n)\ \exp\left(-C_3(n-4-K_n q_n)\min(\lambda_n, \delta_n^2)\right),$$

for some constant $0 < C_3 < \infty$. Further, note that $\lambda_n = -\frac{1}{9}\log(1-c_n^2) \sim c_n^2/9$ as $c_n \to 0$, and by assumptions (A5) and (A6), $c_n^{-2} = \mathcal{O}(n^{2d_2})$ and $\delta_n^{-2} = \mathcal{O}(n^{2d_1})$. Thus

$$\sup_{i,j,S\in\mathbf{S}_{i,j}^{K_n q_n}} \mathbb{P}(E_{nij|S}) \leq \mathcal{O}\left((n - K_n q_n)\ \exp(-C_4(n-K_n q_n)n^{-2\max(d_1,d_2)})\right), \tag{8}$$

for some constant $0 < C_4 < \infty$. Therefore, by combining (7) and (8), we get

$$\begin{aligned}
&\mathbb{P}(\hat{\mathcal{C}}_n \neq \mathcal{C}_{n0}, A_n^{\mathsf{c}}) \\
\leq &\sum_{i,j,S\in\mathbf{S}_{i,j}^{K_n q_n}} \mathbb{P}(E_{nij|S}) \\
\leq &\mathcal{O}(p_n^{K_n q_n+2}) \sup_{i,j,S\in\mathbf{S}_{i,j}^{K_n q_n}} \mathbb{P}(E_{nij|S}) \\
\leq &\mathcal{O}\left(p_n^{K_n q_n+2}(n-K_n q_n)\ \exp(-C_4(n-K_n q_n)n^{-2\max(d_1,d_2)})\right) \\
\leq &\mathcal{O}\left(\exp((K_n q_n+2)\log(p_n) + \log(n) - C_4 n^{1-2\max(d_1,d_2)} + C_4 K_n q_n n^{-2\max(d_1,d_2)})\right) \to 0,
\end{aligned}$$

since $C_4 n^{1-2\max(d_1,d_2)}$ dominates all other terms as $p_n = \mathcal{O}(n^a)$ for some constant $0 \leq a < \infty$ (by assumption (A2)), $K_n q_n = \mathcal{O}(n^{1-b_2})$ with $0 < b_2 \leq 1$ (by assumption (A3) and (A5)), and $2\max(d_1, d_2) < b_2$ (by assumptions (A5) and (A6)). This completes the proof. □

## 9.8 Proof of Lemma 5.3 of the main text

Since $X_i$ and $X_j$ are not connected by a path in $\mathcal{C}_0$, we have $X_i \perp_{\mathcal{G}_0} X_j \mid \{X_r : r \in S\}$ for all $S \subseteq \{1,\dots,p\} \setminus \{i,j\}$. Therefore, we have $\rho_{ij|S} = 0$ for all $S \subseteq \{1,\dots,p\} \setminus \{i,j\}$, since $\mathcal{G}_0$ is a perfect map of the distribution. Thus, it follows from Lemma 5.2 of the main text that the oracle score of a DAG in which $X_i$ and $X_j$ are not adjacent cannot be improved by adding an edge between $X_i$ and $X_j$. This completes the proof, since a $\delta$-optimal oracle version of (AR)GES improves the score at every step of its forward phase (see Definition 5.3 of the main text). □

## 9.9 Proof of Theorem 5.3 of the main text

As we discussed in the main text, it is sufficient to prove that the output of the forward phase of the oracle version of (AR)GES is $\mathcal{C}_0$ when $\mathcal{G}_0$ is a polytree. Further, we will only prove the result for GES as Theorem 9.1 below, and we note that the same proof holds for ARGES. In order to prove Theorem 9.1, we prepare ourselves with the following definitions and lemmas.

**Lemma 9.6.** *If $\mathcal{G}$ is a polytree, $\mathcal{C} = \text{CPDAG}(\mathcal{G})$ and $X_i \to X_j$ is a directed edge in $\mathcal{C}$, then for each $X_r \in \mathbf{Adj}_{\mathcal{C}}(X_j)$, $X_r$ and $X_j$ are connected by a directed edge in $\mathcal{C}$.*

*Proof.* Suppose $X_i \to X_j - X_r$ in $\mathcal{C}$. Then it follows Lemma 1 of Meek [1995] that $X_i \to X_k$ in $\mathcal{C}$, as $\mathcal{C}$ is a CPDAG. This is a contradiction, since skeleton $\mathcal{C}$ is a tree. □

**Definition 9.1.** *A CPDAG $\mathcal{C}$ is said to be contained in $\mathcal{C}_0$ if the following conditions hold:*

1. $\text{skeleton}(\mathcal{C}) \subseteq \text{skeleton}(\mathcal{C}_0)$*, and*
2. *if the path $\pi_{\mathcal{C}}(X_i, X_j, X_k)$ exists, then $\pi_{\mathcal{C}}(X_i, X_j, X_k)$ is a v-structure if and only if $\pi_{\mathcal{C}_0}(X_i, X_j, X_k)$ is a v-structure.*

**Lemma 9.7.** *If $\mathcal{C}$ is contained in $\mathcal{C}_0$ and $X_i \to X_j$ is a directed edge in $\mathcal{C}$, then $X_i \to X_j$ is a directed edge in $\mathcal{C}_0$.*

*Proof.* We construct $\mathcal{P}$ from $\mathcal{C}$ by removing orientations of all directed edges in $\mathcal{C}$ that are not part of a v-structure. Similarly, we construct $\mathcal{P}_0$ from $\mathcal{C}_0$. By Definition 9.1 it holds that $\text{skeleton}(\mathcal{P}) \subseteq \text{skeleton}(\mathcal{P}_0)$ and if $X_i \to X_j$ is a directed edge in $\mathcal{P}$, then $X_i \to X_j$ is a directed edge in $\mathcal{P}_0$.

Theorem 3 of Meek [1995] asserts that $\mathcal{C}$ and $\mathcal{C}_0$ can be constructed from $\mathcal{P}$ and $\mathcal{P}_0$ respectively by applying the orientation rules R1, R2 and R3 defined in Section 2.1.2 of Meek [1995]. It is easy to verify from the definitions of R1, R2 and R3 that $\mathcal{C}$ cannot contain a directed edge that is not oriented in the same way in $\mathcal{C}_0$, as $\mathcal{P}$ is a subgraph of $\mathcal{P}_0$. □

We will assume that the forward phase of GES starts with a CPDAG $\mathcal{C}_1$ which is contained in $\mathcal{C}_0$. Note that the empty graph, which is often used as a starting point of the GES algorithm, is contained in $\mathcal{C}_0$. We denote the sequence of CPDAGs obtained in the forward phase (including the initial CPDAG) by $\{\mathcal{C}_1, \mathcal{C}_2, \ldots\}$. Chickering [2002] defined a move from $\mathcal{C}_t$ to $\mathcal{C}_{t+1}$ through the Insert operator, which is defined as follows.

**Definition 9.2.** *(*Insert *operator, Definition 12 of Chickering [2002]) A node $X_r$ is said to be a neighbor of $X_j$ $\mathcal{C}$ if $X_r - X_j$ is an undirected edge in $\mathcal{C}$. For non-adjacent nodes $X_i$ and $X_j$ in $\mathcal{C}$, and for any subset $\mathbf{T}$ of the neighbors of $X_j$ that are not adjacent to $X_i$,* $\text{Insert}(X_i, X_j, \mathbf{T})$ *modifies $\mathcal{C}$ by inserting the directed edge $X_i \to X_j$ and for each $X_r \in \mathbf{T}$, directing the previously undirected edge between $X_r$ and $X_j$ as $X_r \to X_j$.*

The Insert operator acts on a CPDAG $\mathcal{C}$ and produces a candidate PDAG that has exactly one more edge than $\mathcal{C}$. A DAG $\mathcal{G}$ is a consistent extension of a PDAG $\mathcal{P}$ if $\mathcal{G}$ can be constructed from $\mathcal{P}$ by orienting its undirected edges without creating a directed cycle or a new v-structure. $\text{Insert}(X_i, X_j, \mathbf{T})$ is said to be a valid operation on $\mathcal{C}$ if the resulting PDAG has a consistent extension $\mathcal{G} = (\mathbf{X}, E)$ such that the DAG $\mathcal{G}' = (\mathbf{X}, E \setminus \{X_i \to X_j\})$ is in the Markov equivalence class of $\mathcal{C}$. Theorem 15 of Chickering [2002] provides necessary and sufficient conditions for an Insert operation to be valid. To state this result, we first define a semi-directed path and the notation $\mathbf{NA}_{\mathcal{C}}(X_j, X_i)$.

**Definition 9.3.** *A semi-directed path from $X_j$ to $X_i$ in a PDAG is a path from $X_j$ to $X_i$ such that each edge on the path is either undirected or directed away from $X_j$.*

**Notation 9.1.** $\mathbf{NA}_{\mathcal{C}}(X_j, X_i)$ *denotes the set of nodes that are connected to $X_j$ by an undirected edge and connected to $X_i$ by a directed edge in $\mathcal{C}$.*

**Lemma 9.8.** *(Theorem 15 of Chickering [2002]) Let $X_i$ and $X_j$ be non-adjacent nodes in $\mathcal{C}$ and let $\mathbf{T}$ be a subset of the neighbors of $X_j$ that are not adjacent to $X_i$.* $\text{Insert}(X_i, X_j, \mathbf{T})$ *is a valid operation on $\mathcal{C}$ if and only if in $\mathcal{C}$*

1. $\mathbf{NA}_{\mathcal{C}}(X_j, X_i) \cup \mathbf{T}$ *is a clique, and*
2. *every semi-directed path from $X_j$ to $X_i$ contains a node in* $\mathbf{NA}_{\mathcal{C}}(X_j, X_i) \cup \mathbf{T}$.

**Corollary 9.2.** *If $\mathcal{G}$ is a polytree and* $\mathcal{C} = \text{CPDAG}(\mathcal{G})$, *then* $\text{Insert}(X_i, X_j, \mathbf{T})$ *is a valid operation on $\mathcal{C}$ only if one of the following conditions hold:*

1. $\mathbf{NA}_{\mathcal{C}}(X_j, X_i) \cup \mathbf{T} = \emptyset$;
2. $|\mathbf{NA}_{\mathcal{C}}(X_j, X_i) \cup \mathbf{T}| = 1$ *and* $\mathbf{Pa}_{\mathcal{C}}(X_j) = \emptyset$.

*Proof.* By Lemma 9.8, $\text{Insert}(X_i, X_j, \mathbf{T})$ is a valid operation on $\mathcal{C}$ only if $\mathbf{NA}_{\mathcal{C}}(X_j, X_i) \cup \mathbf{T}$ is a clique in $\mathcal{C}$. Since all nodes in $\mathbf{NA}_{\mathcal{C}}(X_j, X_i) \cup \mathbf{T}$ are adjacent to $X_j$ in $\mathcal{C}$, the fact that $\mathbf{NA}_{\mathcal{C}}(X_j, X_i) \cup \mathbf{T}$ is a clique implies that $\mathbf{NA}_{\mathcal{C}}(X_j, X_i) \cup \mathbf{T} \cup X_j$ is a clique as well. Therefore, $\mathbf{NA}_{\mathcal{C}}(X_j, X_i) \cup \mathbf{T} \cup X_j$ must contain at most two nodes for $\text{Insert}(X_i, X_j, \mathbf{T})$ to be a valid operation on $\mathcal{C}$, as skeleton($\mathcal{C}$) is a tree. This implies $|\mathbf{NA}_{\mathcal{C}}(X_j, X_i) \cup \mathbf{T}| \leq 1$. Further, if $|\mathbf{NA}_{\mathcal{C}}(X_j, X_i) \cup \mathbf{T}| = 1$, then there is a node $X_r$ that is connected to $X_j$ by an undirected edge. By Lemma 9.6, this is impossible unless $\mathbf{Pa}_{\mathcal{C}}(X_j) = \emptyset$. □

**Notation 9.2.** *For $\mathbf{S} \subseteq \mathbf{X} \setminus \{X_i, X_j\}$, we now denote the partial correlation between $X_i$ and $X_j$ given $\mathbf{S}$ by $\rho_{ij|\mathbf{S}}$. We use the shorthand $\rho_{ij}$ and $\rho_{ij|k}$ to denote $\rho_{ij|\emptyset}$ and $\rho_{ij|\{X_k\}}$ respectively. (Note that this is a slight change in notation, as we previously denoted the partial correlation between $X_i$ and $X_j$ given $\mathbf{S}$ using the notation $\rho_{ij|S}$ with $S = \{r : X_r \in \mathbf{S}\}$ being the corresponding set of indices.)*

**Lemma 9.9.** *Assume that the distribution of $\mathbf{X}$ is multivariate Gaussian and assume that $\mathcal{G}_0$ is a perfect map. Let $X_k \in \mathbf{X} \setminus \{X_i, X_j\}$ and let $\mathbf{S} \subseteq \mathbf{X} \setminus \{X_i, X_j\}$.*

**(i)** *If $X_i \perp_{\mathcal{G}_0} X_j \mid \emptyset$, $|\rho_{ij|k}| \leq |\rho_{ik|j}|$ and the inequality is strict when $\rho_{ij|k} \neq 0$.*

**(ii)** *If $X_i \perp_{\mathcal{G}_0} X_j \mid \mathbf{S} \cup \{X_k\}$ for some $X_k \notin \mathbf{S}$, then $|\rho_{ij|\mathbf{S}}| \leq |\rho_{ik|\mathbf{S}}|$ and the inequality is strict when $\rho_{ij|\mathbf{S}} \neq 0$.*

**(iii)** *If $X_i \perp_{\mathcal{G}_0} X_r \mid \mathbf{S}' \cup \{X_j\}$ for all $X_r \in \mathbf{S}$ and $\mathbf{S}' \subseteq \mathbf{S} \setminus \{X_r\}$, then $|\rho_{ij|\mathbf{S}}| \leq |\rho_{ij}|$ and the inequality is strict when $\rho_{ir} \neq 0$ for some $X_r \in \mathbf{S}$.*

**(iv)** *If $X_i \perp_{\mathcal{G}_0} X_r \mid \mathbf{S}'$ for all $X_r \in \mathbf{S}$ and $\mathbf{S}' \subseteq \mathbf{S} \setminus \{X_r\}$, then $|\rho_{ij|\mathbf{S}}| \geq |\rho_{ij}|$ for all $X_j \notin \mathbf{S}$ and the inequality is strict when $\rho_{jr} \neq 0$ for some $X_r \in \mathbf{S}$.*

*Proof.* We will mainly use the well-known formula for expressing an $(r+1)$-th order partial correlation in terms of $r$-th order partial correlations:

$$\rho_{i_1 i_2|\mathbf{U}\cup\{X_{i_3}\}} = \frac{\rho_{i_1 i_2|\mathbf{U}} - \rho_{i_1 i_3|\mathbf{U}}\ \rho_{i_2 i_3|\mathbf{U}}}{\sqrt{\left(1-\rho^2_{i_1 i_3|\mathbf{U}}\right)\left(1-\rho^2_{i_2 i_3|\mathbf{U}}\right)}}, \tag{9}$$

where $\mathbf{U} \subseteq \mathbf{X} \setminus \{X_{i_1}, X_{i_2}, X_{i_3}\}$ such that $|\mathbf{U}| = r$, for $0 \le r \le p-3$.

**Proof of (i):**
Since $\mathcal{G}_0$ is a perfect map, $X_i \perp_{\mathcal{G}_0} X_j \mid \emptyset$ implies $\rho_{ij} = 0$. By applying (9) twice with $(i_1, i_2, i_3, \mathbf{U}) = (i, k, j, \emptyset)$ and with $(i_1, i_2, i_3, \mathbf{U}) = (k, j, i, \emptyset)$ and by using $\rho_{ij} = 0$, we obtain

$$\rho_{ik|j} = \frac{\rho_{ik}}{\sqrt{1-\rho^2_{kj}}} \text{ and } \rho_{kj|i} = \frac{\rho_{kj}}{\sqrt{1-\rho^2_{ik}}}.$$

Therefore,

$$|\rho_{ij|k}| = \frac{|\rho_{ij} - \rho_{ik}\rho_{kj}|}{\sqrt{(1-\rho^2_{ik})(1-\rho^2_{kj})}} = \frac{|\rho_{ik}\rho_{kj}|}{\sqrt{(1-\rho^2_{ik})(1-\rho^2_{kj})}} = |\rho_{ik|j}||\rho_{kj|i}| \le |\rho_{ik|j}|.$$

Since $\rho_{ij|k} \neq 0$ implies that both $\rho_{ik|j}$ and $\rho_{kj|i}$ are non-zero, the above inequality is strict when $\rho_{ij|k} \neq 0$.

**Proof of (ii):**
Since $\mathcal{G}_0$ is a perfect map, $X_i \perp_{\mathcal{G}_0} X_j \mid \mathbf{S} \cup \{X_k\}$ implies $\rho_{ij|\mathbf{S}\cup\{X_k\}} = 0$. By applying (9) with $(i_1, i_2, i_3, \mathbf{U}) = (i, j, k, \mathbf{S})$ and by using $\rho_{ij|\mathbf{S}\cup\{X_k\}} = 0$, we obtain

$$|\rho_{ij|\mathbf{S}}| = |\rho_{ik|\mathbf{S}}| \cdot |\rho_{kj|\mathbf{S}}| \le |\rho_{ik|\mathbf{S}}|.$$

Since $\rho_{ij|\mathbf{S}} \neq 0$ implies that both $\rho_{ik|\mathbf{S}}$ and $\rho_{kj|\mathbf{S}}$ are non-zero, the above inequality is strict when $\rho_{ij|\mathbf{S}} \neq 0$.

**Proof of (iii):**
Let $\mathbf{S} = \{X_{r_1}, \ldots, X_{r_s}\}$, excluding the trivial case $\mathbf{S} = \emptyset$. We define $\mathbf{S}_{-[m]} = \{X_{r_{m+1}}, \ldots, X_{r_s}\}$, for $m = 1, \ldots, s-1$. Further, let $\mathbf{S}_{-[0]} = \mathbf{S}$ and let $\mathbf{S}_{-[s]} = \emptyset$. Since $\mathcal{G}_0$ is a perfect map, $X_i \perp_{\mathcal{G}_0} X_{r_m} \mid \mathbf{S}_{-[m]} \cup \{X_j\}$ implies $\rho_{ir_m|\mathbf{S}_{-[m]}\cup\{X_j\}} = 0$, for $m = 1, \ldots, s$. By applying (9) with $(i_1, i_2, i_3, \mathbf{U}) = (i, r_m, j, \mathbf{S}_{-[m]})$ and by using $\rho_{ir_m|\mathbf{S}_{-[m]}\cup\{X_j\}} = 0$, we obtain

$$\rho_{ir_m|\mathbf{S}_{-[m]}} = \rho_{ij|\mathbf{S}_{-[m]}}\ \rho_{jr_m|\mathbf{S}_{-[m]}}, \quad \text{for } m = 1, \ldots, s. \tag{10}$$

By applying (9) with $(i_1, i_2, i_3, \mathbf{U}) = (i, j, r_m, \mathbf{S}_{-[m]})$ and by using (10), we obtain

$$|\rho_{ij|\mathbf{S}_{-[m-1]}}| = \frac{|\rho_{ij|\mathbf{S}_{-[m]}}|\left(1-\rho^2_{jr_m|\mathbf{S}_{-[m]}}\right)}{\sqrt{\left(1-\rho^2_{ir_m|\mathbf{S}_{-[m]}}\right)\left(1-\rho^2_{jr_m|\mathbf{S}_{-[m]}}\right)}} = |\rho_{ij|\mathbf{S}_{-[m]}}|\frac{\sqrt{1-\rho^2_{jr_m|\mathbf{S}_{-[m]}}}}{\sqrt{1-\rho^2_{ir_m|\mathbf{S}_{-[m]}}}} \le |\rho_{ij|\mathbf{S}_{-[m]}}|. \tag{11}$$

The last inequality follows from (10), which implies $|\rho_{ir_m|\mathbf{S}_{-[m]}}| \leq |\rho_{jr_m|\mathbf{S}_{-[m]}}|$. Moreover, it also follows from (10) that the inequality in (11) is strict if $\rho_{ir_m|\mathbf{S}_{-[m]}} \neq 0$. Finally, by applying (11) successively for $m = 1, \dots, s$, we obtain

$$|\rho_{ij|\mathbf{S}}| \leq |\rho_{ij|\mathbf{S}_{-[1]}}| \leq \cdots \leq |\rho_{ij|\mathbf{S}_{-[s-1]}}| \leq |\rho_{ij}|,$$

where the last inequality is strict if $\rho_{ir_s} \neq 0$.

**Proof of (iv):**
Let $\mathbf{S} = \{X_{r_1}, \dots, X_{r_s}\}$, excluding the trivial case $\mathbf{S} = \emptyset$. We define $\mathbf{S}_{[m]} = \{X_{r_1}, \dots, X_{r_m}\}$, for $m = 1, \dots, s$, and $\mathbf{S}_{[0]} = \emptyset$. Since $\mathcal{G}_0$ is a perfect map, $X_i \perp_{\mathcal{G}_0} X_{r_m} \mid \mathbf{S}_{[m-1]}$ implies $\rho_{ir_m|\mathbf{S}_{[m-1]}} = 0$, for $m = 1, \dots, s$. By applying (9) with $(i_1, i_2, i_3, \mathbf{U}) = (i, j, r_m, \mathbf{S}_{[m-1]})$ and by using $\rho_{ir_m|\mathbf{S}_{[m-1]}} = 0$, we obtain

$$|\rho_{ij|\mathbf{S}_{[m]}}| = |\rho_{ij|\mathbf{S}_{[m-1]} \cup \{X_{r_m}\}}| = \frac{|\rho_{ij|\mathbf{S}_{[m-1]}}|}{\sqrt{1 - \rho^2_{jr_m|\mathbf{S}_{[m-1]}}}} \geq |\rho_{ij|\mathbf{S}_{[m-1]}}|. \tag{12}$$

Note that the inequality in (12) is strict if $\rho_{jr_m|\mathbf{S}_{[m-1]}} \neq 0$. Finally, by applying (11) successively for $m = s, \dots, 1$, we obtain

$$|\rho_{ij|\mathbf{S}}| \geq |\rho_{ij|\mathbf{S}_{[s-1]}}| \geq \cdots \geq |\rho_{ij|\mathbf{S}_{[1]}}| \geq |\rho_{ij}|,$$

where the last inequality is strict if $\rho_{jr_1} \neq 0$. □

**Theorem 9.1.** *Assume that the distribution of* $\mathbf{X}$ *is multivariate Gaussian. If* $\mathcal{G}_0$ *is a polytree and the forward phase of the oracle version of GES starts with a CPDAG that is contained in* $\mathcal{C}_0$*, then the output of the forward phase of the oracle version of GES with scoring criterion* $\mathcal{S}^*_\lambda$ *is* $\mathcal{C}_0$*, for any* $\lambda$ *satisfying* $\lambda < -\frac{1}{2}\log(1 - \rho^2_{ij|\mathbf{S}})$ *for all* $i, j \in \{1, \dots, p\}$ *and* $\mathbf{S} \subseteq \{X_1, \dots, X_p\} \setminus \{X_i, X_j\}$ *such that* $|\mathbf{S}| \leq \max_{1 \leq i \leq p} |\mathbf{Adj}_{\mathcal{C}_0}(X_i)|$.

*Proof.* Let $\mathcal{C}^f$ be the output of the forward phase of the oracle version of GES. First, we argue that it is sufficient to show that $\mathcal{C}^f$ is contained in $\mathcal{C}_0$ (see Definition 9.1). Since $\mathcal{C}^f$ is an independence map of $\mathcal{C}_0$ (see the proof of Theorem 5.1), skeleton$(\mathcal{C}^f) \supseteq$ skeleton$(\mathcal{C}_0)$. Therefore, if $\mathcal{C}^f$ is contained in $\mathcal{C}_0$, then they must have the same skeleton and the same set of v-structures and hence they must be identical.

Next, we denote the sequence of CPDAGs obtained in the forward phase by $\{\mathcal{C}_1, \mathcal{C}_2, \dots\}$, where we assumed that $\mathcal{C}_1$ is contained in $\mathcal{C}_0$. Therefore, it is sufficient to show that $\mathcal{C}_{t+1}$ is contained in $\mathcal{C}_0$ given that $\mathcal{C}_t$ is contained in $\mathcal{C}_0$.

Let $(X_i, X_j, \mathbf{T})$ be the triple such that Insert$(X_i, X_j, \mathbf{T})$ yielded the move from $\mathcal{C}_t$ to $\mathcal{C}_{t+1}$. This implies that Insert$(X_i, X_j, \mathbf{T})$ is a valid operation on $\mathcal{C}_t$, meaning that the undirected edges in the PDAG obtained by applying Insert$(X_i, X_j, \mathbf{T})$ on $\mathcal{C}_t$ can be oriented without creating a directed cycle or a new v-structure. Moreover, by definition, the Insert$(X_i, X_j, \mathbf{T})$ operation leads to the best improvement (which must be non-zero) upon the score $\mathcal{S}^*_\lambda(\mathcal{C}_t, F)$ among all possible valid Insert operations on $\mathcal{C}_t$.

We argue below that if $\mathbf{NA}_{\mathcal{C}_t}(X_j, X_i) \neq \emptyset$, then Insert$(X_i, X_j, \mathbf{T})$ does not improve upon $\mathcal{S}^*_\lambda(\mathcal{C}_t, F)$. To this end, note that Corollary 16 of Chickering [2002] and Lemma 5.1 of the main text imply that

$$\mathcal{S}^*_\lambda(\mathcal{C}_{t+1}, F) - \mathcal{S}^*_\lambda(\mathcal{C}_t, F) = \frac{1}{2}\log(1 - \rho^2_{ij|\mathbf{Z}'(i,j,\mathbf{T},\mathcal{C}_t)}) + \lambda,$$

where $\mathbf{Z}'(i, j, \mathbf{T}, \mathcal{C}_t) := \mathbf{NA}_{\mathcal{C}_t}(X_j, X_i) \cup \mathbf{T} \cup \mathbf{Pa}_{\mathcal{C}_t}(X_j)$.

Suppose $X_r \in \mathbf{NA}_{\mathcal{C}_t}(X_j, X_i)$. By definition (see Notation 9.1), $X_r$ is connected to $X_i$ by a directed edge in $\mathcal{C}_t$ and $X_r$ is connected to $X_j$ by an undirected edge in $\mathcal{C}_t$. Then it follows from Lemma 9.6 that the edge between $X_r$ and $X_i$ must be directed towards $X_i$. Hence, $\pi_{\mathcal{C}_t}(X_i, X_r, X_j)$ is a non-collider path such that $X_i$ and $X_j$ are not adjacent (as skeleton($\mathcal{C}_t$) is a tree). This implies $\pi_{\mathcal{C}_0}(X_i, X_r, X_j)$ is a non-collider path as well, since $\mathcal{C}_t$ is contained in $\mathcal{C}_0$. Further, note that $\pi_{\mathcal{C}_0}(X_i, X_r, X_j)$ is the only path between $X_i$ and $X_j$, since skeleton($\mathcal{C}_0$) is a tree. Therefore, $X_i \perp_{\mathcal{G}_0} X_j \mid \mathbf{Z}'(i, j, \mathbf{T}, \mathcal{C}_t)$, and we have $\rho_{ij|\mathbf{Z}'(i,j,\mathbf{T},\mathcal{C}_t)} = 0$.

Therefore, without loss of generality, we assume $\mathbf{NA}_{\mathcal{C}_t}(X_j, X_i) = \emptyset$, and we define

$$\mathbf{Z}(r, \mathbf{T}) := \mathbf{Pa}_{\mathcal{C}_t}(X_r) \cup \mathbf{T},$$

where we omitted the dependence of $\mathcal{C}_t$ from the left hand side for notational convenience.

We complete the proof by showing that if $\mathcal{C}_{t+1}$ is not contained in $\mathcal{C}_0$, then either $|\rho_{ij|\mathbf{Z}(j,\mathbf{T})}| = 0$ or $|\rho_{ij|\mathbf{Z}(j',\mathbf{T}')}| > |\rho_{ij|\mathbf{Z}(j,\mathbf{T})}|$ for some triple $(X_{i'}, X_{j'}, \mathbf{T}')$ such that $X_{i'}$ and $X_{j'}$ are not connected by a path in $\mathcal{C}_t$, $\mathbf{T}'$ is a subset of neighbors of $X_j$, and $|\mathbf{T}'| \leq 1$. Note that the latter case leads to a contradiction as $X_{i'}$ and $X_{j'}$ are not connected by a path in $\mathcal{C}_t$ implies that $\mathbf{NA}_{\mathcal{C}_t}(X_{j'}, X_{i'}) = \emptyset$ and that Insert$(X_{i'}, X_{j'}, \mathbf{T}')$ is a valid operation for any subset $\mathbf{T}'$ of neighbors of $X_j$ such that $|\mathbf{T}'|$ is a clique (see Lemma 9.8).

It is easy to verify that $C_{t+1}$ is not contained in $\mathcal{C}_0$ if and only if at least one of the following conditions hold:

**(C1)** $X_i$ and $X_j$ are not adjacent in $\mathcal{C}_0$,

**(C2)** there exists $X_r \in \mathbf{Z}(j, \mathbf{T})$ such that $\pi_{\mathcal{C}_0}(X_i, X_j, X_r)$ is a non-collider path,

**(C3)** there exists $X_r \in \mathbf{Adj}_{\mathcal{C}_t}(X_j) \setminus \mathbf{Z}(j, \mathbf{T})$ such that $X_i \to X_j \leftarrow X_r$ is a v-structure in $\mathcal{C}_0$, and

**(C4)** there exists $X_s \in \mathbf{Adj}_{\mathcal{C}_t}(X_i)$ such that $X_s \to X_i \leftarrow X_j$ is a v-structure in $\mathcal{C}_0$.

Note that **(C1)** implies skeleton($\mathcal{C}_{t+1}$) $\not\subseteq$ skeleton($\mathcal{C}_0$). **(C2)** implies that there is a v-structure in $\mathcal{C}_{t+1}$ that is not a v-structure in $\mathcal{C}_0$. **(C3)** and **(C4)** implies that there is a v-structure in $\mathcal{C}_0$ that is not a v-structure in $\mathcal{C}_t$.

**Suppose (C1) holds**:

Since skeleton($\mathcal{C}_0$) is a tree, there exists a unique path $\pi_{\mathcal{C}_0}(X_i, \ldots, X_j)$ between $X_i$ and $X_k$ in $\mathcal{C}_0$. Let $X_k$ be the node that precedes $X_j$ on $\pi_{\mathcal{C}_0}(X_i, \ldots, X_k, X_j)$.

**Case 1: All pairs of successive nodes on $\pi_{\mathcal{C}_0}(X_i, \ldots, X_k, X_j)$ are adjacent in $\mathcal{C}_t$.**

We show that $\mathbf{Z}(j, \mathbf{T})$ blocks the only path $\pi_{\mathcal{G}_0}(X_i, \ldots, X_k, X_j)$ between $X_i$ and $X_j$ in $\mathcal{G}_0$, and hence $\rho_{ij|\mathbf{Z}(j,\mathbf{T})} = 0$.

Suppose $X_k \in \mathbf{Z}(j, \mathbf{T})$. Then the edge between $X_k$ and $X_j$ in $\mathcal{C}_t$ is either undirected or directed towards $X_j$. Hence, $\pi_{\mathcal{C}_t}(X_i, X_r, X_j)$ is a non-collider path such that $X_i$ and $X_j$ are not adjacent (as skeleton($\mathcal{C}_t$) is a tree). This implies $\pi_{\mathcal{C}_0}(X_i, X_r, X_j)$ is a non-collider path as well, since $\mathcal{C}_t$ is contained in $\mathcal{C}_0$. Therefore, $\mathbf{Z}(j, \mathbf{T})$ blocks the path $\pi_{\mathcal{G}_0}(X_i, \ldots, X_k, X_j)$.

Suppose $X_k \notin \mathbf{Z}(j, \mathbf{T})$. Then it follows from the second condition Lemma 9.8 that $\pi_{\mathcal{C}_t}(X_i, \ldots, X_k, X_j)$ is not a semi-directed path from $X_j$ to $X_i$, i.e., the path must contain an edge $X_r \to X_s$ that is directed towards $X_j$. Therefore, it follows from Lemma 9.6 that either that the subpath $\pi_{\mathcal{C}_t}(X_r, \ldots, X_k, X_j)$ is a directed path from $X_r$ to $X_j$ or that $\pi_{\mathcal{C}_t}(X_r, \ldots, X_k, X_j)$ contains a collider. The former is impossible, since $X_k \notin \mathbf{Pa}_{\mathcal{C}_t}(X_j)$. Thus $\pi_{\mathcal{C}_t}(X_i, \ldots, X_k, X_j)$ contains a collider, and by Lemma 9.7, $\pi_{\mathcal{C}_0}(X_i, \ldots, X_k, X_j)$ must contain the same collider. Thus $\mathbf{Z}(j, \mathbf{T})$ blocks $\pi_{\mathcal{G}_0}(X_i, \ldots, X_k, X_j)$, since $\mathbf{Z}(j, \mathbf{T})$ does not intersect the path as $X_k \notin \mathbf{Z}(j, \mathbf{T})$.

**Case 2: There is a pair of successive nodes on $\pi_{\mathcal{C}_0}(X_i, \ldots, X_k, X_j)$ that is not adjacent in $\mathcal{C}_t$ and $X_k \in \mathbf{Z}(j, \mathbf{T})$.**

We show that if $\rho_{ij|\mathbf{Z}(j,\mathbf{T})} \neq 0$, then $|\rho_{ij|\mathbf{Z}(j,\mathbf{T})}| < |\rho_{ik|\mathbf{Z}(k,\{X_j\})}|$.

To this end, note that $\rho_{ij|\mathbf{Z}(j,\mathbf{T})} \neq 0$ and $X_k \in \mathbf{Z}(j, \mathbf{T})$ imply that $X_k$ is a collider on the path $\pi_{\mathcal{C}_0}(X_i, \ldots, X_k, X_j)$. Therefore, by Lemma 9.7, the edge between $X_k$ and $X_j$ in $\mathcal{C}_t$ is either directed towards $X_k$ or undirected. The former is impossible, since $X_k \in \mathbf{Z}(j, \mathbf{T})$. Thus $X_k \in \mathbf{T}$, and hence, we have $\mathbf{Z}(j, \mathbf{T}) = \{X_k\}$ (by Corollary 9.2).

Further, since $X_k$ and $X_j$ are connected by an undirected edge, by Lemma 9.6, we have $\mathbf{Z}(k, \{X_j\}) = \{X_j\}$. Therefore, $|\rho_{ij|\mathbf{Z}(j,\mathbf{T})}| < |\rho_{ik|\mathbf{Z}(k,\{X_j\})}|$ follows from the first result of Lemma 9.9, since $X_k$ is a collider on $\pi_{\mathcal{C}0(X_i,\ldots,X_j)}$ implies that $X_i \perp_{\mathcal{G}_0} X_j \mid \emptyset$.

**Case 3: There is a pair of successive nodes on $\pi_{\mathcal{C}_0}(X_i, \ldots, X_k, X_j)$ that is not adjacent in $\mathcal{C}_t$ and $X_k \notin \mathbf{Z}(j, \mathbf{T})$.**

We assume that $\rho_{ij|\mathbf{Z}(j,\mathbf{T})} \neq 0$. Note that $X_k \notin \mathbf{Z}(j, \mathbf{T})$ implies that $\mathbf{Z}(j, \mathbf{T})$ does not intersect $\pi_{\mathcal{C}_0}(X_i, \ldots, X_k, X_j)$. Therefore, we must have that

$$\pi_{\mathcal{C}_0}(X_i, \ldots, X_j) \text{ is a non-collider path.} \tag{13}$$

Therefore, since skeleton($\mathcal{C}_0$) is a tree, we have

$$X_i \perp_{\mathcal{G}_0} X_j \mid \mathbf{Z}(j, \mathbf{T}) \cup \{X_k\}. \tag{14}$$

**Subcase 3(a): $X_k$ and $X_j$ are non-adjacent in $\mathcal{C}_t$.** From (14) and the second result of Lemma 9.9 with $(i,j,k,\mathbf{S}) = (j,i,k,\mathbf{Z}(j,\mathbf{T}))$ it follows that $|\rho_{ij|\mathbf{Z}(j,\mathbf{T})}| < |\rho_{kj|\mathbf{Z}(j,\mathbf{T})}|$.

**Subcase 3(b): $X_k - X_j$ is an undirected edge in $\mathcal{C}_t$.** We show that $|\rho_{ij|\mathbf{Z}(j,\mathbf{T})}| < |\rho_{ik|\mathbf{Z}(k,\emptyset)}|$.

From (14) and the second result of Lemma 9.9 with $(i,j,k,\mathbf{S}) = (i,j,k,\mathbf{Z}(j,\mathbf{T}))$, we have

$$|\rho_{ij|\mathbf{Z}(j,\mathbf{T})}| < |\rho_{ik|\mathbf{Z}(j,\mathbf{T})}|. \tag{15}$$

Thus it remains to show that $|\rho_{ik|\mathbf{Z}(j,\mathbf{T})}| \leq |\rho_{ik|\mathbf{Z}(k,\emptyset)}|$.

Since $X_k - X_j$ is an undirected edge in $\mathcal{C}_t$, we have $\mathbf{Pa}_{\mathcal{C}_t}(X_j) = \mathbf{Pa}_{\mathcal{C}_t}(X_k) = \emptyset$ (by Lemma 9.6). Therefore, we have $\mathbf{Z}(j,\mathbf{T}) = \mathbf{T}$ and $\mathbf{Z}(k,\emptyset) = \emptyset$. By Lemma 9.2, $\mathbf{T}$ is either the empty set or a singleton set. Note that $|\rho_{ik|\mathbf{Z}(j,\mathbf{T})}| \leq |\rho_{ik|\mathbf{Z}(k,\emptyset)}|$ trivially holds for $\mathbf{T} = \emptyset$. Thus we assume $\mathbf{Z}(j,\mathbf{T}) = \mathbf{T} = \{X_r\}$, for some node $X_r$. Since skeleton$(\mathcal{C}_t) \subseteq$ skeleton$(\mathcal{C}_0)$, $X_j$ and $X_r$ are adjacent in $\mathcal{C}_0$. By (13), $X_k$ is a not a collider on $\pi_{\mathcal{C}_0}(X_i,\dots,X_k,X_j,X_r)$, and hence, $X_k$ is a not a collider on the corresponding path in $\mathcal{G}_0$. This implies $X_i \perp_{\mathcal{G}_0} X_r \mid \{X_k\}$. By applying the third result of Lemma 9.9 with $(i,j,\mathbf{S}) = (i,k,\{X_r\})$, we obtain

$$|\rho_{ik|\mathbf{Z}(j,\mathbf{T})}| = |\rho_{ik|r}| \leq |\rho_{ik}| = |\rho_{ik|\mathbf{Z}(k,\emptyset)}|.$$

**Subcase 3(c): $X_k \leftarrow X_j$ is a directed edge in $\mathcal{C}_t$.** We show that

$$|\rho_{ij|\mathbf{Z}(j,\mathbf{T})}| < |\rho_{ik|\mathbf{Z}(j,\mathbf{T})}| \leq |\rho_{ik}| \leq |\rho_{ik|\mathbf{Z}(i,\emptyset)}|.$$

The first inequality is the same as (15). The second inequality follows from the third result of Lemma 9.9 with $(i,j,\mathbf{S}) = (i,k,\mathbf{Z}(j,\mathbf{T}))$. To see this, let $X_r \in \mathbf{Z}(j,\mathbf{T})$, excluding the trivial case $\mathbf{Z}(j,\mathbf{T}) = \emptyset$. Then it follows from (13) that $X_k$ is a not a collider on the unique path $\pi_{\mathcal{C}_0}(X_i,\dots,X_k,X_j,X_r)$ between $X_i$ and $X_r$. This implies $X_i \perp_{\mathcal{G}_0} X_r \mid X_k \cup \mathbf{S}'$ for $X_r \in \mathbf{Z}(j,\mathbf{T})$ and $\mathbf{S}' \subseteq \mathbf{Z}(j,\mathbf{T}) \setminus \{X_r\}$.

Finally, we argue below that the third inequality follows from the fourth result of Lemma 9.9 with $(i,j,\mathbf{S}) = (k,i,\mathbf{Z}(i,\emptyset))$. Let $X_s \in \mathbf{Z}(i,\emptyset) = \mathbf{Pa}_{\mathcal{C}_t}(X_i)$, excluding the trivial case $\mathbf{Pa}_{\mathcal{C}_t}(X_i) = \emptyset$. Since $\mathcal{C}_t$ is contained in $\mathcal{C}_0$ and $X_k \leftarrow X_j$ is a directed edge in $\mathcal{C}_t$, it follows from Lemma 9.7 that $X_k \leftarrow X_j$ is a directed edge in $\mathcal{C}_0$ as well. Then it follows from (13) and Lemma 9.6 that all edges in $\pi_{\mathcal{C}_0}(X_i,\dots,X_k,X_j)$ are directed towards $X_i$. Since $X_s \in \mathbf{Pa}_{\mathcal{C}_t}(X_i)$ and $\mathbf{Pa}_{\mathcal{C}_t}(X_i) \subseteq \mathbf{Pa}_{\mathcal{C}_0}(X_i)$ (see Lemma 9.7), $X_i$ is a collider on $\pi_{\mathcal{C}_0}(X_s,X_i,\dots,X_k)$. Therefore, $X_k \perp_{\mathcal{G}_0} X_s \mid \mathbf{S}'$ for $X_s \in \mathbf{Z}(i,\emptyset)$ and $\mathbf{S}' \subseteq \mathbf{Z}(i,\emptyset) \setminus \{X_s\}$, as $\mathbf{Z}(i,\emptyset) \setminus \{X_s\} \subseteq \mathbf{Pa}_{\mathcal{G}_0}(X_i) \subseteq \mathbf{Nd}_{\mathcal{G}_0}(X_i)$. Hence, we can apply the fourth result of Lemma 9.9 with $(i,j,\mathbf{S}) = (k,i,\mathbf{Z}(i,\emptyset))$.

**Suppose (C1) does not hold but (C2) holds**:

Fix $X_r \in \mathbf{Z}(j,\mathbf{T})$ such that $\pi_{\mathcal{C}_0}(X_i,X_j,X_r)$ is a non-collider path.

**Case 1:** $X_r \in \mathbf{Pa}_{\mathcal{C}_t}(X_j)$**.** We show below that

$$|\rho_{ij|\mathbf{Z}(j,\mathbf{T})}| < |\rho_{ij}| \leq |\rho_{ij|\mathbf{Z}(i,\emptyset)}|. \tag{16}$$

Since $\mathbf{Pa}_{\mathcal{C}_t}(X_j) \neq \emptyset$, Corollary 9.2 implies that $\mathbf{Z}(j,\mathbf{T}) = \mathbf{Pa}_{\mathcal{C}_t}(X_j)$. Further, $X_r \in \mathbf{Pa}_{\mathcal{C}_t}(X_j)$ implies $X_r \in \mathbf{Pa}_{\mathcal{C}_0}(X_j)$ (see Lemma 9.7). Hence, $\pi_{\mathcal{C}_0}(X_i, X_j, X_r)$ is a non-collider path in $\mathcal{C}_0$ implying that $\pi_{\mathcal{C}_0}(X_i, X_j, X_r)$ is a directed path from $X_r$ to $X_i$ for all $X_r \in \mathbf{Pa}_{\mathcal{C}_t}(X_j)$ (see Lemma 9.6). Therefore, $X_i \perp_{\mathcal{G}_0} X_r \mid \mathbf{S}' \cup \{X_j\}$ for all $X_r \in \mathbf{Pa}_{\mathcal{C}_t}(X_j)$ and $\mathbf{S}' \subseteq \mathbf{Pa}_{\mathcal{C}_t}(X_j) \setminus \{X_r\}$. Thus the first inequality in (16) follows from the third result of Lemma 9.9 with $(i,j,\mathbf{S}) = (i,j,\mathbf{Pa}_{\mathcal{C}_t}(X_j))$. Note that the inequality is strict since $\rho_{ir} \neq 0$ for each $X_r \in \mathbf{Pa}_{\mathcal{C}_t}(X_j)$ (as $\pi_{\mathcal{C}_0}(X_i, X_j, X_r)$ is a non-collider path).

The second inequality in (16) follows from the fourth result of Lemma 9.9 with $(i,j,\mathbf{S}) = (j,i,\mathbf{Z}(i,\emptyset))$. To see this, note that $X_r \in \mathbf{Z}(i,\emptyset) = \mathbf{Pa}_{\mathcal{C}_t}(X_i)$ implies that $X_r \in \mathbf{Pa}_{\mathcal{C}_t}(X_i)$ (see Lemma 9.7). Therefore, $\pi_{\mathcal{C}_0}(X_r, X_i, X_j)$ is a v-structure for all $X_r \in \mathbf{Z}(i,\emptyset)$. Hence, we have $X_j \perp_{\mathcal{G}_0} X_r \mid \mathbf{S}'$ for all $X_r \in \mathbf{Z}(i,\emptyset)$ and $\mathbf{S}' \subseteq \mathbf{Z}(i,\emptyset) \setminus \{X_r\}$.

**Case 2:** $X_r \in \mathbf{T}$**.** We show that

$$|\rho_{ij|\mathbf{Z}(j,\mathbf{T})}| = |\rho_{ij|r}| < |\rho_{ij}| = |\rho_{ij|\mathbf{Z}(j,\emptyset)}|.$$

Since $X_r \in \mathbf{T}$, Corollary 9.2 imply that $\mathbf{Z}(j,\mathbf{T}) = \mathbf{T} = \{X_r\}$ and $\mathbf{Z}(j,\emptyset) = \emptyset$. Finally, $|\rho_{ij|r}| < |\rho_{ij}|$ follows from the third results of Lemma 9.9 with $(i,j,\mathbf{S}) = (i,j,\{X_r\})$, since $\pi_{\mathcal{G}_0}(X_i, X_j, X_r)$ is a non-collider path implying that $X_i \perp_{\mathcal{G}_0} X_r \mid \{X_j\}$ and that $\rho_{ir} \neq 0$.

**Suppose (C1) and (C2) do not hold but (C3) holds**:

Fix $X_r \in \mathbf{Adj}_{\mathcal{C}_t}(X_j) \setminus \mathbf{Z}(j,\mathbf{T})$ such that $X_i \to X_j \leftarrow X_r$ is a v-structure in $\mathcal{C}_0$. We show that $X_j$ and $X_r$ are connected by an undirected edge in $\mathcal{C}_t$ (this allows us to consider Insert$(X_i, X_j, \{X_r\})$) and

$$|\rho_{ij|\mathbf{Z}(j,\mathbf{T})}| = |\rho_{ij}| < |\rho_{ij|r}| = |\rho_{ij|\mathbf{Z}(j,\{X_r\})}|.$$

First, note that Lemma 9.7 implies that the edge between $X_j$ and $X_r$ in $\mathcal{C}_t$ must be either oriented towards $X_j$ or undirected. The former is impossible, since $X_r \notin \mathbf{Pa}_{\mathcal{C}_t}(X_j)$. Therefore, $X_j$ and $X_r$ are connected by an undirected edge in $\mathcal{C}_t$.

Next, suppose $\mathbf{Z}(j,\mathbf{T}) \neq \emptyset$. Let $X_{r'} \in \mathbf{Z}(j,\mathbf{T})$. Since **(C2)** does not hold, $\pi_{\mathcal{C}_0}(X_i, X_j, X_{r'})$ is a v-structure. Therefore, $\pi_{\mathcal{C}_0}(X_r, X_j, X_{r'})$ is a v-structure but $\pi_{\mathcal{C}_t}(X_r, X_j, X_{r'})$ is not a v-structure (as we have shown that $X_j$ and $X_r$ are connected by an undirected edge in $\mathcal{C}_t$). This is a contradiction as $\mathcal{C}_t$ is contained in $\mathcal{C}_0$. Thus $\mathbf{Z}(j,\mathbf{T}) = \emptyset$. This implies $\mathbf{Pa}_{\mathcal{C}_t}(X_j) = \emptyset$ and hence $\mathbf{Z}(j,\{X_r\}) = \{X_r\}$.

Finally, $|\rho_{ij}| < |\rho_{ij|r}|$ follows from the fourth result of Lemma 9.9 with $(i,j,\mathbf{S}) = (i,j,\{X_r\})$, as $X_i \to X_j \leftarrow X_r$ is a v-structure in $\mathcal{G}_0$.

**Suppose (C1), (C2) and (C2) do not hold but (C4) holds**:

Fix $X_s \in \mathbf{Adj}_{\mathcal{C}_t}(X_i)$ such that $X_s \to X_i \leftarrow X_j$ is a v-structure in $\mathcal{C}_0$. Let $\mathbf{T}' = \{X_s\} \setminus \mathbf{Pa}_{\mathcal{C}_t}(X_i)$. We show that

$$|\rho_{ij|\mathbf{Z}(j,\mathbf{T})}| = |\rho_{ij}| < |\rho_{ij|\mathbf{Z}(i,\mathbf{T}')}|. \tag{17}$$

Suppose $\mathbf{Z}(j, \mathbf{T}) \neq \emptyset$. Let $X_r \in \mathbf{Z}(j, \mathbf{T})$. Since $X_j \in \mathbf{Pa}_{\mathcal{C}_0}(X_i)$, $\pi_{\mathcal{C}_0}(X_i, X_j, X_r)$ is a non-collider path. This contradicts the fact **(C2)** does not hold. Thus, we have $\mathbf{Z}(j, \mathbf{T}) = \emptyset$, and hence $|\rho_{ij|\mathbf{Z}(j,\mathbf{T})}| = |\rho_{ij}|$.

Note that $\mathbf{Z}(i, \mathbf{T}') = \{X_s\} \cup \mathbf{Pa}_{\mathcal{C}_t}(X_i) \subseteq \mathbf{Pa}_{\mathcal{C}_0}(X_i)$. This implies $X_i$ is a collider on $\pi_{\mathcal{C}_0}(X_{s'}, X_i, X_j)$ for each $X_{s'} \in \mathbf{Z}(i, \mathbf{T}')$. Therefore, $X_j \perp_{\mathcal{G}_0} X_{s'} \mid \mathbf{S}'$ for $X_{s'} \in \mathbf{Z}(i, \mathbf{T}')$ and $\mathbf{S}' \subseteq \mathbf{Z}(i, \mathbf{T}') \setminus \{X_{s'}\}$. Thus the inequality in (17) follows from the fourth result of Lemma 9.9 with $(i, j, \mathbf{S}) = (j, i, \mathbf{Z}(i, \mathbf{T}'))$. Note that the inequality is strict, since $X_s \in \mathbf{Z}(i, \mathbf{T}')$ and $\rho_{is} \neq 0$. □

## 9.10 Proof of Theorem 5.4 of the main text

In order to prove Theorem 5.4 of the main text, we modify Lemma 9.9 as follows.

**Lemma 9.10.** *Assume that the distribution of* $\mathbf{X}$ *is multivariate Gaussian and assume that* $\mathcal{G}_0$ *is a perfect map. Assume (A6) with* $K = 1$ *and (A7). Let* $\delta < \min((1 - M)c,\ c')$ *where* $M$ *and* $c$ *are given by (A6) and* $c'$ *is given by (A7). Let* $X_k \in \mathbf{X} \setminus \{X_i, X_j\}$ *and let* $\mathbf{S} \subseteq \mathbf{X} \setminus \{X_i, X_j\}$.

**(i)** *If* $X_i \perp_{\mathcal{G}_0} X_j \mid \emptyset$, $|\rho_{ij|k}| \leq |\rho_{ik|j}|$. *Further, if* $\rho_{ij|k} \neq 0$, *then* $\big||\rho_{ij|k}| - |\rho_{ik|j}|\big| > \delta$.

**(ii)** *If* $X_i \perp_{\mathcal{G}_0} X_j \mid \mathbf{S} \cup \{X_k\}$ *for some* $X_k \notin \mathbf{S}$, *then* $|\rho_{ij|\mathbf{S}}| \leq |\rho_{ik|\mathbf{S}}|$. *Further, if* $\rho_{ij|\mathbf{S}} \neq 0$, *then* $\big||\rho_{ij|\mathbf{S}}| - |\rho_{ik|\mathbf{S}}|\big| > \delta$.

**(iii)** *If* $X_i \perp_{\mathcal{G}_0} X_r \mid \mathbf{S}' \cup \{X_j\}$ *for all* $X_r \in \mathbf{S}$ *and* $\mathbf{S}' \subseteq \mathbf{S} \setminus \{X_r\}$, *then* $|\rho_{ij|\mathbf{S}}| \leq |\rho_{ij}|$. *Further, if* $\rho_{ir} \neq 0$ *and* $\pi_{\mathcal{G}_0}(X_i, X_j, X_r)$ *is an unshielded triple in* $\mathcal{G}_0$ *for some* $X_r \in \mathbf{S}$, *then* $\big||\rho_{ij|\mathbf{S}}| - |\rho_{ij}|\big| > \delta$.

**(iv)** *If* $X_i \perp_{\mathcal{G}_0} X_r \mid \mathbf{S}'$ *for all* $X_r \in \mathbf{S}$ *and* $\mathbf{S}' \subseteq \mathbf{S} \setminus \{X_r\}$, *then* $|\rho_{ij|\mathbf{S}}| \geq |\rho_{ij}|$ *for all* $X_j \notin \mathbf{S}$. *Further, if* $\rho_{jr} \neq 0$ *and* $\pi_{\mathcal{G}_0}(X_i, X_j, X_r)$ *is an unshielded triple in* $\mathcal{G}_0$ *for some* $X_r \in \mathbf{S}$, *then* $\big||\rho_{ij|\mathbf{S}}| - |\rho_{ij}|\big| > \delta$.

*Proof.*
**Proof of (i):**
Recall that in the proof of Lemma 9.9, we proved the first part of (i) by showing that $|\rho_{ij|k}| = |\rho_{ik|j}| \cdot |\rho_{kj|i}|$. Therefore,

$$\big||\rho_{ij|k}| - |\rho_{ik|j}|\big| = (1 - |\rho_{kj|i}|)|\rho_{ik|j}| > (1 - M)c > \delta,$$

where the second last inequality follows from (A6).

**Proof of (ii):**
We proved the first part of (ii) in Lemma 9.9 and the second part of (ii) follows from similar arguments given in the proof the second part of (i).

**Proof of (iii):**
We proved the first part of (iii) in Lemma 9.9. To prove the second part, we fix $X_r \in \mathbf{S}$ such that $\rho_{ir} \neq 0$ and $\pi_{\mathcal{G}_0}(X_i, X_j, X_r)$ is an unshielded triple in $\mathcal{G}_0$. Recall that in the proof of Lemma 9.9, we showed that $|\rho_{ij|\mathbf{S}}| \leq |\rho_{ij|r}| < |\rho_{ij}|$. Therefore,

$$\big||\rho_{ij|\mathbf{S}}| - |\rho_{ij}|\big| \geq \big||\rho_{ij|r}| - |\rho_{ij}|\big| \geq c' > \delta,$$

where the second last inequality follows from (A7).

**Proof of (iv):**
We proved the first part of (iv) in Lemma 9.9 and the second part of (iv) follows from similar arguments given in the proof the second part of (iii). □

**Proof of Theorem 5.4 of the main text.** We note that Lemma 9.10 makes sure that for each strict inequality $a < b$ (between the absolute values of two partial correlations) used in the proof of Theorem 5.3 of the main text (see the proof of Theorem 9.1 above), we additionally have $|a - b| > \delta$. Therefore, a proof of Theorem 5.4 of the main text can be constructed by repeating the arguments given in the proof of Theorem 9.1 while applying Lemma 9.10 instead of Lemma 9.9. □

## 9.11 Proof of Theorem 6.1 of the main text

As we discussed in Section 6 of the main text, the soundness of $\delta_n$-optimal oracle versions of (AR)GES for a linear SEM follows from Lemma 5.2 and Theorem 5.1 of the main text. Thus we only require to prove an analogue of Corollary 9.1 for linear SEMs with sub-Gaussian distribution (see the proof of Theorem 5.2 of the main text).

We fix $i, j \in \{1, \ldots, p_n\}$ with $i \neq j$ and fix $S \subseteq \{1, \ldots, p_n\} \setminus \{i, j\}$ such that $|S| \leq K_n q_n$. We complete the proof by showing that for any $\delta \in (0, 1)$,

$$\mathbb{P}(|\hat{\rho}_{nij|S} - \rho_{nij|S}| > \delta) \leq 2\exp(-C' n \delta^2), \tag{18}$$

where $C' > 0$ depends only on $C_1$, $C_2$ and $C_3$ given by (A1*) and (A8).

Let $\mathbf{X}'_n$ denote a $q'_n = |S| + 2$ dimensional random vector consisting of $\{X_{ni}, X_{nj}\} \cup \{X_{nr} : r \in S\}$ in some order. Let $\Sigma_n = \text{Cov}(\mathbf{X}'_n)$ and let $\hat{\Sigma}_n$ be the corresponding sample covariance matrix. By analyzing the error propagation from a covariance matrix to a partial correlation, Harris and Drton [2013] obtained the following result.

$$|\hat{\rho}_{nij|S} - \rho_{nij|S}| < C_4 q'_n \, ||\hat{\Sigma}_n - \Sigma_n||_\infty, \tag{19}$$

where $||A||_\infty = \max_{i,j} |A_{ij}|$ and the constant $C_4$ depends only on $C_2$ and $C_3$. Note that Harris and Drton [2013] worked with a correlation matrix instead of a covariance matrix. However,

a straightforward modification of Lemma 6 of Harris and Drton [2013] using the fact that $\min_i (\Sigma_n^{-1})_{ii} \geq 1/C_3$ would lead to (19). Furthermore, we note that a straightforward modification of Lemma 5 of Harris and Drton [2013] leads to

$$|\hat{\rho}_{nij|S} - \rho_{nij|S}| < C_4 \, ||\hat{\Sigma}_n - \Sigma_n||_2.$$

Finally, we apply the following result from the random matrix theory to obtain (18). If $q_n'/n \to 0$ and there is an absolute constant $C_5 > 0$ such that $||\mathbf{X}_n'||_{\psi_2} < C_5$, then for any $\delta \in (0,1)$ and sufficiently large $n$,

$$\mathbb{P}(||\hat{\Sigma}_n - \Sigma_n||_2 > \delta) \leq 2\exp(-C_6 n\delta^2),$$

for some absolute constant $C_6 > 0$ depending on $C_5$ (see Corollary 5.50 of Vershynin [2012]). This completes the proof, since $||\mathbf{X}_n'||_{\psi_2} < C_5$ follows from (A1*) and (A8). □

## 9.12 Proof of Lemma 7.1 of the main text

It is easy to see that $\tilde{\mathcal{S}}_{\lambda_n}(\mathcal{H}_n, \mathcal{D}_n)$ is a decomposable score for any ordering of the directed edges in $\mathcal{H}_n$ in which they are added to the empty graph. Therefore, it suffices to prove the result for the DAG $\mathcal{H}$ that has the vertex set $\{X_1, \dots, X_p\}$ and the edge set $\{X_i \to X_p : i = 1, \dots, k\}$, where we removed the dependency on $n$ from the subscripts for notational convenience.

We define $s(1, \dots, k) := \sum_{r=1}^{k} \log\left(1 - \hat{\rho}^2_{rp|\{1,\dots,r-1\}}\right)$. We complete the proof by showing that $s(1, \dots, k) = s(r_1, \dots, r_k)$ for any permutation $(r_1, \dots, r_k)$ of $(1, \dots, k)$. Let $\hat{\Psi}$ be the submatrix of $\hat{\Sigma}$ that corresponds to $(X_p, X_1, \dots, X_r)$ and let $\hat{\Psi}_{\setminus X_p}$ be the submatrix of $\hat{\Sigma}$ that corresponds to $(X_1, \dots, X_r)$. Then permutation invariance of $s(1, \dots, k) = \log\left(\prod_{r=1}^{k}(1 - \hat{\rho}^2_{rp|\{1,\dots,r-1\}})\right)$ follows from the following identity [Pearson, 1916] and the permutation invariance property of the determinant of a matrix:

$$\prod_{r=1}^{k}(1 - \hat{\rho}^2_{rp|\{1,\dots,r-1\}}) = \frac{|\hat{\Psi}|}{|\hat{\Psi}_{\setminus X_p}|}. \tag{20}$$

Note that if $\hat{\Psi}$ is a sample correlation matrix, then (20) is a well-known identity that expresses a multiple correlation coefficient in terms of partial correlation coefficients. In particular, the right hand side of (20) equals $1 - \hat{r}^2_{p|1,\dots,k}$, where $\hat{r}_{p|1,\dots,k}$ is the multiple correlation coefficient of $X_p$ on $X_1, \dots, X_r$. Interestingly, the proof of (20) given in Pearson [1916] does not require positive definiteness of $\hat{\Psi}$. Hence, the result holds even if $\hat{\Psi}$ is not a positive (semi)definite matrix. This is important because the rank based estimator $\hat{\Sigma}$ defined in Section 7 of the main text may not be a positive (semi)definite matrix. □

## 9.13 Proof of Lemma 7.2 of the main text

Let $\mathcal{H}_n$ and $\mathcal{H}_n'$ be two Markov equivalent DAGs. By Theorem 4 of Chickering [2002], there exists a sequence of covered edge reversals that transforms $\mathcal{H}_n$ to $\mathcal{H}_n'$, where an

edge $X_{ni} \to X_{nk}$ is said to be covered in a DAG $\mathcal{H}_n$ if $\mathbf{Pa}_{\mathcal{H}_n}(X_{nk}) = \mathbf{Pa}_{\mathcal{H}_n}(X_{ni}) \cup \{X_{ni}\}$. Therefore, it suffices to prove the result assuming that $\mathcal{H}_n$ and $\mathcal{H}'_n$ are identical, except that they have opposite orientation of exactly one covered edge. Let $X_{ni} \to X_{nk}$ be the covered edge in $\mathcal{H}_n$ that is oriented as $X_{nk} \to X_{ni}$ in $\mathcal{H}'_n$. Now we construct the DAG $\mathcal{H}^*_n$ by deleting the edge $X_{ni} \to X_{nk}$ from $\mathcal{H}_n$ (or equivalently, by deleting the edge $X_{nk} \to X_{ni}$ from $\mathcal{H}'_n$). We complete the proof by showing that $\tilde{\mathcal{S}}_{\lambda_n}(\mathcal{H}'_n, \mathcal{D}_n) - \tilde{\mathcal{S}}_{\lambda_n}(\mathcal{H}^*_n, \mathcal{D}_n) = \tilde{\mathcal{S}}_{\lambda_n}(\mathcal{H}_n, \mathcal{D}_n) - \tilde{\mathcal{S}}_{\lambda_n}(\mathcal{H}^*_n, \mathcal{D}_n)$, for all $\mathcal{D}_n$. By Definition 7.2,

$$\tilde{\mathcal{S}}_{\lambda_n}(\mathcal{H}_n, \mathcal{D}_n) - \tilde{\mathcal{S}}_{\lambda_n}(\mathcal{H}^*_n, \mathcal{D}_n) = \frac{1}{2}\log(1 - \hat{\rho}^2_{nik|\mathbf{Pa}_{\mathcal{H}^*_n}(k)}) + \lambda_n, \text{ and}$$
$$\tilde{\mathcal{S}}_{\lambda_n}(\mathcal{H}'_n, \mathcal{D}_n) - \tilde{\mathcal{S}}_{\lambda_n}(\mathcal{H}^*_n, \mathcal{D}_n) = \frac{1}{2}\log(1 - \hat{\rho}^2_{nik|\mathbf{Pa}_{\mathcal{H}^*_n}(i)}) + \lambda_n$$

This completes the proof, since the definition of $\mathcal{H}^*_n$ and the fact that $X_{ni} \to X_{nk}$ is a covered edge in $\mathcal{H}_n$ imply $\mathbf{Pa}_{\mathcal{H}^*_n}(k) = \mathbf{Pa}_{\mathcal{H}_n}(k) \setminus \{X_{ni}\} = \mathbf{Pa}_{\mathcal{H}_n}(i) = \mathbf{Pa}_{\mathcal{H}^*_n}(i)$. □

## 9.14 Proof of Theorem 7.1 of the main text

Note that the soundness of $\delta_n$-optimal oracle versions of (AR)GES with the scoring criterion $\tilde{\mathcal{S}}^*_\lambda$ follows from Theorem 5.1 of the main text. Thus the result follows from the proof of Theorem 5.2 of the main text and the following result (cf. Corollary 9.1) given by Harris and Drton [2013].

Let $\{m_n\}$ be sequence such that $m_n/n \to 0$ and let $\mathbf{S}^{m_n}_{i,j} = \{S \subseteq \{1, \dots, p_n\} \setminus \{i, j\} : |S| \leq m_n\}$. Then for any $\delta > 0$ and sufficiently large $n$,

$$\sup_{i,j,S \in \mathbf{S}^{m_n}_{i,j}} \mathbb{P}\left(\left|\hat{\rho}_{nij|S} - \rho_{nij|S}\right| > \delta\right) \leq A \exp\left(-\frac{BC_2^4 n\delta^2}{m_n^2}\right),$$

for some absolute constants $A, B > 0$. □

# References


Chickering, D. M. (1995). A transformational characterization of bayesian network structures. In *UAI 1995*.

Chickering, D. M. (2002). Optimal structure identification with greedy search. *J. Mach. Learn. Res.*, 3:507–554.

Colombo, D. and Maathuis, M. (2014). Order-independent constraint-based causal structure learning. *J. Mach. Learn. Res.*, 15:3741–3782.

Fawcett, T. (2006). An introduction to ROC analysis. *Pattern Recogn. Lett.*, 27:861–874.

Harris, N. and Drton, M. (2013). PC algorithm for nonparanormal graphical models. *J. Mach. Learn. Res.*, 14:3365–3383.

Hauser, A. and Bühlmann, P. (2012). Characterization and greedy learning of interventional Markov equivalence classes of directed acyclic graphs. *J. Mach. Learn. Res.*, 13:2409–2464.

Kalisch, M. and Bühlmann, P. (2007). Estimating high-dimensional directed acyclic graphs with the PC-algorithm. *J. Mach. Learn. Res.*, 8:613–636.

Kalisch, M., Mächler, M., Colombo, D., Maathuis, M., and Bühlmann, P. (2012). Causal inference using graphical models with the R package pcalg. *J. Statist. Software*, 47:1–26.

Lauritzen, S. L. (1996). *Graphical models*, volume 17 of *Oxford Statistical Science Series*. The Clarendon Press Oxford University Press, New York.

Meek, C. (1995). Causal inference and causal explanation with background knowledge. In *UAI 1995*.

Meinshausen, N. and Bühlmann, P. (2006). High-dimensional graphs and variable selection with the Lasso. *Ann. Statist.*, 34:1436–1462.

Nandy, P., Hauser, A., and Maathuis, M. H. (2016). High-dimensional consistency in score-based and hybrid structure learning.

Pearson, K. (1916). On some novel properties of partial and multiple correlation coefficients in a universe of manifold characteristics. *Biometrika*, 11(3):231–238.

Verma, T. and Pearl, J. (1990). Causal networks: Semantics and expressiveness. In *UAI 1990*.

Vershynin, R. (2012). Introduction to the non-asymptotic analysis of random matrices. In *Compressed Sensing: Theory and Applications*, pages 210–268. Cambridge Univ Press.

Yule, G. U. (1907). On the theory of correlation for any number of variables, treated by a new system of notation. *Proc. Roy. Soc. London, Ser. A*, 79:182–193.
